# Supplementary material for: Practical Treatment of Singlet Oxygen with Density-Functional Theory and the Multiplet-Sum Method
Source: arXiv:2107.13056 source file (2021-07-27)
Supplement: Supplementary file 1 [file SI.pdf]

Supplementary Information for

# Practical Treatment of Singlet Oxygen with Density-Functional Theory and the Multiplet-Sum Method


Abraham Ponra
*University of Maroua, Cameroon*
*e-mail: abraponra@yahoo.com*

Anne Justine Etindele
*Higher Teachers Training College, University of Yaounde I, P.O. Box 47, Yaounde, Cameroon*
*e-mail: annetindele@yahoo.fr*

Ousmanou Motapon
*University of Maroua, Cameroon*
*e-mail: omotapon@univ-douala.com*

Mark E. Casida
*Laboratoire de Spectrométrie, Interactions et Chimie théorique (SITh), Département de Chimie Moléculaire (DCM, UMR CNRS/UGA 5250), Institut de Chimie Moléculaire de Grenoble (ICMG, FR2607), Université Grenoble Alpes (UGA) 301 rue de la Chimie, BP 53, F-38041 Grenoble Cedex 9, France*
*e-mail: mark.casida@univ-grenoble-alpes.fr*

# Contents

1 Digitized reference potential energy curves 3

2 Group Theoretic Analysis 4

3 Sample deMon2k Input 12

4 Multiplet sum method potential energy curves 14

5 Tables comparing calculated and experimental atomic and diatomic calculated parameters 23

6 Author Contributions 30

Table 1: $O_2$ potential energy curves from Fig. 1 of Ref. [1] digitized with WebPlotDigitizer [2]. The zero of energy is the vibrational zero-point energy of the ground state.

| $R$ (bohr) | Energy (Ha) | | | $R$ (bohr) | Energy (Ha) | | |
|---|---|---|---|---|---|---|---|
| | $X\,^3\Sigma_g^-$ | $a\,^1\Delta_g$ | $b\,^1\Sigma_g^+$ | | $X\,^3\Sigma_g^-$ | $a\,^1\Delta_g$ | $b\,^1\Sigma_g^+$ |
| 1.7 | 0.29247 | 0.33467 | 0.33185 | 4.2 | 0.18426 | 0.18120 | 0.18426 |
| 1.8 | 0.18075 | 0.22188 | 0.25813 | 4.3 | 0.18571 | 0.18353 | 0.18578 |
| 1.9 | 0.08980 | 0.13237 | 0.16356 | 4.4 | 0.18681 | 0.18466 | 0.18681 |
| 2.0 | 0.03976 | 0.08080 | 0.10942 | 4.5 | 0.18766 | 0.18557 | 0.18766 |
| 2.1 | 0.01050 | 0.04976 | 0.07790 | 4.6 | 0.18829 | 0.18616 | 0.18829 |
| 2.2 | -0.00157 | 0.03736 | 0.06365 | 4.7 | 0.18869 | 0.18674 | 0.18869 |
| 2.3 | -0.00276 | 0.03367 | 0.05777 | 4.8 | 0.18905 | 0.18696 | 0.18905 |
| 2.4 | 0.00125 | 0.03717 | 0.05979 | 4.9 | 0.18924 | 0.18725 | 0.18924 |
| 2.5 | 0.01083 | 0.04452 | 0.06617 | 5.0 | 0.18963 | 0.18747 | 0.18963 |
| 2.6 | 0.02345 | 0.05571 | 0.07520 | 5.1 | 0.18974 | 0.18778 | 0.18974 |
| 2.7 | 0.03699 | 0.06810 | 0.08565 | 5.2 | 0.19001 | 0.18775 | 0.19001 |
| 2.8 | 0.05081 | 0.08012 | 0.09644 | 5.3 | 0.19040 | 0.18788 | 0.19040 |
| 2.9 | 0.06570 | 0.09264 | 0.10734 | 5.4 | 0.19025 | 0.18831 | 0.19025 |
| 3.0 | 0.08143 | 0.10494 | 0.11840 | 5.5 | 0.19027 | 0.18828 | 0.19250 |
| 3.1 | 0.09608 | 0.11663 | 0.12890 | 5.6 | 0.19037 | 0.18804 | 0.19214 |
| 3.2 | 0.10986 | 0.12714 | 0.13814 | 5.7 | 0.19045 | 0.18858 | 0.19181 |
| 3.3 | 0.12276 | 0.13678 | 0.14644 | 5.8 | 0.19033 | 0.18885 | 0.19178 |
| 3.4 | 0.13480 | 0.14545 | 0.15365 | 5.9 | 0.19034 | 0.18966 | 0.19196 |
| 3.5 | 0.14550 | 0.15296 | 0.15999 | 6.0 | 0.19036 | 0.19045 | 0.19206 |
| 3.6 | 0.15459 | 0.15927 | 0.16552 | 6.1 | 0.19039 | 0.18840 | 0.19228 |
| 3.7 | 0.16234 | 0.16498 | 0.17007 | 6.2 | 0.19061 | 0.19061 | 0.19233 |
| 3.8 | 0.16889 | 0.16858 | 0.17387 | 6.3 | 0.19065 | 0.19065 | 0.19237 |
| 3.9 | 0.17434 | 0.17189 | 0.17698 | 6.4 | 0.19067 | 0.19067 | 0.19262 |
| 4.0 | 0.17892 | 0.17540 | 0.18056 | 6.5 | 0.19068 | 0.19068 | 0.19262 |
| 4.1 | 0.18210 | 0.17821 | 0.18210 | 6.6 | 0.19059 | 0.19060 | 0.19264 |

# 1 Digitized reference potential energy curves

We found it particularly convenient to digitize data from Fig. 1 of Ref. [1]. The digitized data of Fig. 1 of Ref. [1] is given in **Table 1**.

Table 2: Character table for the $D_{\infty h}$ point group of homonuclear diatomic molecules. The molecule is assumed to lie along the $z$-axis.

| $D_{\infty h}$ | $E$ | $2C_\infty$ | $\cdots$ | $\infty\sigma_v$ | $i$ | $2S_\infty$ | $\cdots$ | $\infty C_2'$ | functions |
|---|---|---|---|---|---|---|---|---|---|
| $A_{1g} = \Sigma_g^+$ | +1 | +1 | $\cdots$ | +1 | +1 | +1 | $\cdots$ | +1 | $x^2+y^2$, $z^2$ |
| $A_{2g} = \Sigma_g^-$ | +1 | +1 | $\cdots$ | -1 | +1 | +1 | $\cdots$ | -1 | $R_z$ |
| $E_{1g} = \Pi_g$ | +2 | $+2\cos(\phi)$ | $\cdots$ | 0 | +2 | $-2\cos(\phi)$ | $\cdots$ | 0 | $(R_x, R_y)$, $(xy, yz)$ |
| $E_{2g} = \Delta_g$ | +2 | $+2\cos(2\phi)$ | $\cdots$ | 0 | +2 | $+2\cos(2\phi)$ | $\cdots$ | 0 | $(x^2-y^2, xy)$ |
| $E_{3g} = \Phi_g$ | +2 | $+2\cos(3\phi)$ | $\cdots$ | 0 | +2 | $-2\cos(3\phi)$ | $\cdots$ | 0 | |
| $E_{ng}$ | +2 | $+2\cos(n\phi)$ | $\cdots$ | 0 | +2 | $(-1)^n 2\cos(n\phi)$ | $\cdots$ | 0 | |
| $\vdots$ | $\vdots$ | $\vdots$ | $\vdots$ | $\vdots$ | $\vdots$ | $\vdots$ | $\vdots$ | $\vdots$ | $\vdots$ |
| $A_{1u} = \Sigma_u^+$ | +1 | +1 | $\cdots$ | +1 | -1 | -1 | $\cdots$ | -1 | $z$, $z^3$, $z(x^2+y^2)$ |
| $A_{2u} = \Sigma_u^-$ | +1 | +1 | $\cdots$ | -1 | -1 | -1 | $\cdots$ | +1 | |
| $E_{1u} = \Pi_u$ | +2 | $+2\cos(\phi)$ | $\cdots$ | 0 | -2 | $+2\cos(\phi)$ | $\cdots$ | 0 | $(x, y)$, $(xz^2, yz^2)$, $[x(x^2+y^2), y(x^2+y^2)]$ |
| $E_{2u} = \Delta_u$ | +2 | $+2\cos(2\phi)$ | $\cdots$ | 0 | -2 | $-2\cos(2\phi)$ | $\cdots$ | 0 | $[xyz, z(x^2-y^2)]$ |
| $E_{3u} = \Phi_u$ | +2 | $+2\cos(3\phi)$ | $\cdots$ | 0 | -2 | $+2\cos(3\phi)$ | $\cdots$ | 0 | $[y(3x^2-y^2), x(x^2-3y^2)]$ |
| $E_{nu}$ | +2 | $+2\cos(n\phi)$ | $\cdots$ | 0 | -2 | $(-1)^{n+1} 2\cos(n\phi)$ | $\cdots$ | 0 | |
| $\vdots$ | $\vdots$ | $\vdots$ | $\vdots$ | $\vdots$ | $\vdots$ | $\vdots$ | $\vdots$ | $\vdots$ | $\vdots$ |

## 2 Group Theoretic Analysis

The construction of the SALCs of the real (i.e., cartesian) MOs may be carried out using the $D_{\infty h}$ character table (**Table 2**) which assumes that the molecule is aligned along the $z$-axis. An elegant treatment might involve constructing the projectors onto each representation (which should involve some integrals for this infinite group) and applying them to project out the wave functions for each representation. However this was not judged necessary. Instead we will just verify one-by-one that the results given in **Fig. 1** (repeated here from the main article for the reader's convenience) are consistent with the $D_{\infty h}$ character table.

**Triplet ($^3\Sigma_g^-$) Oxygen** This is the ground state of $^3O_2$. From our first-year University course work, we expect the part of the wavefunction outside of the closed shell to be represented by the determinant $|\pi_x^*, \pi_y^*|$. The character table says that this wave function should have the same symmetry as a rotation around the $z$ axis ($R_z$). To verify this, we need two symmetry operations, namely rotation by an angle $\phi$ around and reflection through a vertical plane passing through the two nuclei and at an angle of $\phi$ to the $x$-axis. As for $R_z$, the rotation should leave the wave function invariant (character +1) while the reflection should change the sign of the wave function (character -1).

Let us begin with the rotation. Rotating the orbitals by $\phi$ in the positive (i.e., counter clockwise) direction is equivalent to rotating the $(x, y)$ coordinate system by $\phi$ in the negative (i.e., clockwise) direction. Before rotation, we have

$$\begin{aligned} x &= r\cos\theta \\ y &= r\sin\theta\,. \end{aligned} \quad (1)$$

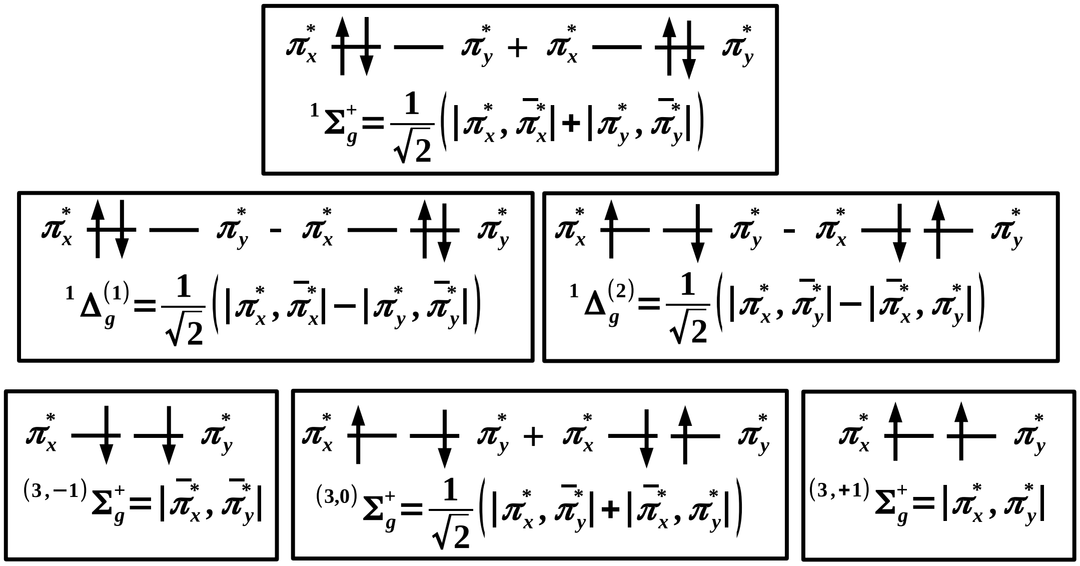


Figure 1: Practical representation of the lowest three electronic states of $O_2$ using real-valued MOs.

After rotation, we have

$$\begin{aligned} x' &= r\cos(\theta+\phi) = r\cos\theta\cos\phi - r\sin\theta\sin\phi \\ &= x\cos\phi - y\sin\phi \\ y' &= r\sin(\theta+\phi) = r\cos\theta\sin\phi + r\sin\theta\cos\phi \\ &= x\sin\phi + y\cos\phi\,. \end{aligned} \tag{2}$$

It is convenient to write this as

$$\begin{pmatrix} x' \\ y' \end{pmatrix} = \mathbf{R}(\phi)\begin{pmatrix} x' \\ y' \end{pmatrix} \tag{3}$$

where the rotation matrix

$$\mathbf{R}(\phi) = \begin{bmatrix} \cos\phi & -\sin\phi \\ \sin\phi & \cos\phi \end{bmatrix}. \tag{4}$$

The inverse rotation is given by

$$\mathbf{R}(-\phi) = \begin{bmatrix} \cos\phi & \sin\phi \\ -\sin\phi & \cos\phi \end{bmatrix}, \tag{5}$$

as is easily checked by verifying that

$$\mathbf{R}(\phi)\mathbf{R}(-\phi) = \mathbf{1}\,. \tag{6}$$

Let us turn now to reflection through a line at a positive angle $\phi$ in the $(x,y)$-plane. If $\phi = 0$, then the line is just the $x$-axis and the transformation is,

$$\begin{aligned} x' &= x \\ y' &= -y\,. \end{aligned} \tag{7}$$

Let us write this as

$$\begin{pmatrix} x' \\ y' \end{pmatrix} = \sigma_v(0) \begin{pmatrix} x \\ y \end{pmatrix} , \tag{8}$$

where

$$\sigma_v(0) = \begin{bmatrix} 1 & 0 \\ 0 & -1 \end{bmatrix} . \tag{9}$$

To find the reflection matrix at an arbitrary angle, we can use an old group theoretician's trick called conjugation: we will first rotate by $-\phi$ to move the reflection line onto the $x$-axis, then we will reflect through the $x$-axis, and finally we will undo the rotation to place the reflection line in its orginal position. The new matrix is,

$$\begin{aligned} \sigma_v(\phi) &= \mathbf{R}(\phi)\sigma_v(0)\mathbf{R}(-\phi) \\ &= \begin{bmatrix} \cos\phi & -\sin\phi \\ \sin\phi & \cos\phi \end{bmatrix} \begin{bmatrix} 1 & 0 \\ 0 & -1 \end{bmatrix} \begin{bmatrix} \cos\phi & \sin\phi \\ -\sin\phi & \cos\phi \end{bmatrix} \\ &= \begin{bmatrix} \cos^2\phi - \sin^2\phi & 2\cos\phi\sin\phi \\ 2\cos\phi\sin\phi & \sin^2\phi - \cos^2\phi \end{bmatrix} \\ &= \begin{bmatrix} \cos(2\phi) & \sin(2\phi) \\ \sin(2\phi) & -\cos(2\phi) \end{bmatrix} . \end{aligned} \tag{10}$$

Hence reflection through an arbrary $\sigma_v$ plane gives,

$$\begin{aligned} x' &= x\cos(2\phi) + y\sin(2\phi) \\ y' &= x\sin(2\phi) - y\cos(2\phi) . \end{aligned} \tag{11}$$

We may see how the wave function $|\pi_x^*, \pi_y^*|$ transforms under rotation around the bond axis:

$$\begin{aligned} |\pi_{x'}^*, \pi_{y'}^*| &= |\pi_x^*\cos\phi - \pi_y^*\sin\phi, \pi_x^*\sin\phi + \pi_y^*\cos\phi| \\ &= |\pi_x^*, \pi_x^*|\cos\phi\sin\phi + |\pi_x^*, \pi_y^*|\cos^2\phi - |\pi_y^*, \pi_x^*|\sin^2\phi + |\pi_y^*, \pi_y^*|\sin\phi\cos\phi \\ &= 0 + |\pi_x^*, \pi_y^*|\cos^2\phi + |\pi_x^*, \pi_y^*|\sin^2\phi + 0 \\ &= |\pi_x^*, \pi_y^*| \left(\cos^2\phi + \sin^2\phi\right) \\ &= |\pi_x^*, \pi_y^*| . \end{aligned} \tag{12}$$

The wave function is indeed invariant with respect to a rotation around the $z$ axis, consistent with the +1 character in the $2C_\infty$ column.

We may now see how the wave function $|\bar{\pi}_x^*, \bar{\pi}_y^*|$ changes upon reflection through an arbitrary $\sigma_v$ axis:

$$\begin{aligned} |\pi_{x'}^*, \pi_{y'}^*| &= |\pi_x^*\cos(2\phi) + \pi_y^*\sin(2\phi), \pi_x^*\sin(2\phi) - \pi_y^*\cos(2\phi)| \\ &= |\pi_x^*, \pi_x^*|\cos(2\phi)\sin(2\phi) - |\pi_x^*, \pi_y^*|\cos^2(2\phi) + |\pi_y^*, \pi_x^*|\sin^2(2\phi) - |\pi_y^*, \pi_y^*|\sin(2\phi)\cos(2\phi) \\ &= 0 - |\pi_x^*, \pi_y^*|\cos^2(2\phi) - |\pi_x^*, \pi_y^*|\sin^2(2\phi) + 0 \\ &= -|\pi_x^*, \pi_y^*| \left(\cos^2(2\phi) + \sin^2(2\phi)\right) \\ &= -|\pi_x^*, \pi_y^*| , \end{aligned} \tag{13}$$

so the wave function changes sign upon arbitrary reflection through a mirror plane containing the two nuclei. This is why there is a -1 character in the $\infty\sigma_v$ column of the character table.

As everything seems to work fine for the spatial wave function, we now only need to recall that every triplet is three-fold spin degenerate. That is, there are three wave functions, differing only by the value of $M_S = -1, 0, +1$ which have the same energy if we neglect any magnetic field effects. These three $\Psi_{S,M_S}$ wave functions are energetically degenerate because they factor into the same antisymmetric spatial part times one of the three different possible symmetric spin parts:

$$\begin{aligned}
\Psi_{1,1} &= |\pi_x^*, \pi_y^*| \\
&= \left[\frac{1}{\sqrt{2}}\left(\pi_x^*(\vec{r}_1)\pi_y^*(\vec{r}_2) - \pi_y^*(\vec{r}_1)\pi_x^*(\vec{r}_2)\right)\right](\alpha_1\alpha_2) \\
\Psi_{1,0} &= \frac{1}{\sqrt{2}}\left(|\pi_x^*, \bar{\pi}_y^*| + |\bar{\pi}_x^*, \pi_y^*|\right) \\
&= \left[\frac{1}{\sqrt{2}}\left(\pi_x^*(\vec{r}_1)\pi_y^*(\vec{r}_2) - \pi_y^*(\vec{r}_1)\pi_x^*(\vec{r}_2)\right)\right]\left[\frac{1}{\sqrt{2}}(\alpha_1\beta_2 + \beta_1\alpha_2)\right] \\
&= \left[\frac{1}{\sqrt{2}}\left(\pi_x^*(\vec{r}_1)\pi_y^*(\vec{r}_2) - \pi_y^*(\vec{r}_1)\pi_x^*(\vec{r}_2)\right)\right](\alpha_1\alpha_2) \\
\Psi_{1,-1} &= |\bar{\pi}_x^*, \bar{\pi}_y^*| \\
&= \left[\frac{1}{\sqrt{2}}\left(\pi_x^*(\vec{r}_1)\pi_y^*(\vec{r}_2) - \pi_y^*(\vec{r}_1)\pi_x^*(\vec{r}_2)\right)\right](\beta_1\beta_2)\ .
\end{aligned} \tag{14}$$

Here the overbar indicates spin $\beta = \downarrow$ otherwise the spin function associated with the orbital is $\alpha = \uparrow$. The three ${}^3\Sigma_g^-$ wavefunctions are shown in the bottom row of Fig. 1. Note the multideterminantal nature of the ${}^{(3,0)}\Sigma_g^-$ state.

For completeness we should verify what happens to $\Psi_{1,0}$ under rotation and reflection.

Rotation:

$$\begin{aligned}
\hat{R}(\phi)\Psi_{1,0} &= \frac{1}{\sqrt{2}}\left(|\pi_{x'}^*\,\bar{\pi}_{y'}^*| + |\bar{\pi}_{x'}^*\,\pi_{y'}^*|\right) \\
&= \frac{1}{\sqrt{2}}\left(|\pi_x^*\cos\phi - \pi_y^*\sin\phi, \bar{\pi}_x^*\sin\phi + \bar{\pi}_y^*\cos\phi| + |\bar{\pi}_x^*\cos\phi - \bar{\pi}_y^*\sin\phi, \pi_x^*\sin\phi + \pi_y^*\cos\phi|\right) \\
&= \frac{1}{\sqrt{2}}\left(|\pi_x^*, \bar{\pi}_x^*|\cos\phi\sin\phi + |\pi_x^*, \bar{\pi}_y^*|\cos^2\phi - |\pi_y^*, \bar{\pi}_x^*|\sin^2\phi - |\pi_y^*, \bar{\pi}_y^*|\sin\phi\cos\phi\right) \\
&+ \frac{1}{\sqrt{2}}\left(|\bar{\pi}_x^*, \pi_x^*|\cos\phi\sin\phi + |\bar{\pi}_x^*, \pi_y^*|\cos^2\phi - |\bar{\pi}_y^*, \pi_x^*|\sin^2\phi - |\bar{\pi}_y^*, \pi_y^*|\cos\phi\sin\phi\right) \\
&= \frac{1}{\sqrt{2}}\left(|\pi_x^*\,\bar{\pi}_y^*| + |\bar{\pi}_x^*\,\pi_y^*|\right) \\
&= \Psi_{1,0}
\end{aligned} \tag{15}$$

Reflection:

$$\begin{aligned}
\hat{\sigma}_v(\phi)\Psi_{1,0} &= \frac{1}{\sqrt{2}}\left(|\pi^*_{x'}\,\bar{\pi}^*_{y'}| + |\bar{\pi}^*_{x'}\,\pi^*_{y'}|\right) \\
&= \frac{1}{\sqrt{2}}|\pi^*_x\cos(2\phi) + \pi^*_y\sin(2\phi), \bar{\pi}^*_x\sin(2\phi) - \bar{\pi}^*_y\cos(2\phi)| \\
&+ \frac{1}{\sqrt{2}}|\bar{\pi}^*_x\cos(2\phi) + \bar{\pi}^*_y\sin(2\phi), \pi^*_x\sin(2\phi) - \pi^*_y\cos(2\phi)| \\
&= \frac{1}{\sqrt{2}}\left(|\pi^*_x, \bar{\pi}^*_x|\cos(2\phi)\sin(2\phi) - |\pi^*_x, \bar{\pi}^*_y|\cos^2(2\phi) + |\pi^*_y, \bar{\pi}^*_x|\sin^2(2\phi) - |\pi^*_y, \bar{\pi}^*_y|\cos(2\phi)\sin(2\phi)\right) \\
&+ \frac{1}{\sqrt{2}}\left(|\bar{\pi}^*_x\pi^*_x|\cos(2\phi)\sin(2\phi) - |\bar{\pi}^*_x, \pi^*_y|\cos^2(2\phi) + |\bar{\pi}^*_y, \pi^*_x|\sin^2(2\phi)| - |\bar{\pi}^*_y, \pi^*_y|\cos(2\phi)\sin(2\phi)\right) \\
&= -\frac{1}{\sqrt{2}}\left(|\pi^*_x, \bar{\pi}^*_y| + |\bar{\pi}^*_x, \pi^*_y|\right) \\
&= -\Psi_{1,0}
\end{aligned} \tag{16}$$

So the $\Psi_{1,0}$ wave function does indeed transform according to the $\Sigma^-_g$ representation.

**Singlet Sigma Oxygen** There are two low-lying singlet excited states of oxygen, namely ${}^1\Delta_g$ and ${}^1\Sigma^+_g$. Singlet oxygen (${}^1O_2$) usually refers to the lower-energy ${}^1\Delta_g$ state. However we will start with the mathematically-simpler ${}^1\Sigma^+_g$ state here whose configuration outside the closed-shell is shown on the top row of Fig. 1. According to the character table, this wave function should transform like $x^2 + y^2$. Its wave function is

$$\Psi = \frac{1}{\sqrt{2}}\left(|\pi^*_x, \bar{\pi}^*_x| + |\pi^*_y, \bar{\pi}^*_y|\right) . \tag{17}$$

Let us check that it transforms correctly under rotation and reflection.

Rotation:

$$\begin{aligned}
\hat{R}(\phi)\Psi &= \frac{1}{\sqrt{2}}\left(|\pi^*_{x'}, \bar{\pi}^*_{x'}| + |\pi^*_{y'}, \bar{\pi}^*_{y'}|\right) \\
&= \frac{1}{\sqrt{2}}|\pi^*_x\cos\phi - \pi^*_y\sin\phi, \bar{\pi}^*_x\cos\phi - \bar{\pi}^*_y\sin\phi| \\
&+ \frac{1}{\sqrt{2}}|\pi^*_x\sin\phi + \pi^*_y\cos\phi, \bar{\pi}^*_x\sin\phi + \bar{\pi}^*_y\cos\phi| \\
&= \frac{1}{\sqrt{2}}\left(|\pi^*_x, \bar{\pi}^*_x|\cos^2\phi - |\pi^*_x, \bar{\pi}^*_y|\cos\phi\sin\phi - |\pi^*_y, \bar{\pi}^*_x|\cos\phi\sin\phi + |\pi^*_y, \bar{\pi}^*_y|\sin^2\phi\right) \\
&+ \frac{1}{\sqrt{2}}\left(|\pi^*_x, \bar{\pi}^*_x|\sin^2\phi + |\pi^*_x, \bar{\pi}^*_y|\cos\phi\sin\phi + |\pi^*_y, \bar{\pi}^*_x|\cos\phi\sin\phi + |\pi^*_y, \bar{\pi}^*_y|\cos^2\phi\right) \\
&= \frac{1}{\sqrt{2}}\left(|\pi^*_x, \bar{\pi}^*_x| + |\pi^*_y, \bar{\pi}^*_y|\right) \\
&= \Psi
\end{aligned} \tag{18}$$

Reflection:

$$
\begin{aligned}
\hat{\sigma}_v(\phi)\Psi &= \frac{1}{\sqrt{2}}\left(|\pi^*_{x'},\bar{\pi}^*_{x'}| + |\pi^*_{y'},\bar{\pi}^*_{y'}|\right) \\
&= \frac{1}{\sqrt{2}}|\pi^*_x\cos(2\phi) + \pi^*_y\sin(2\phi), \bar{\pi}^*_x\cos(2\phi) + \bar{\pi}^*_x\sin(2\phi)| \\
&+ \frac{1}{\sqrt{2}}|\pi^*_x\sin(2\phi) - \pi^*_y\cos(2\phi), \bar{\pi}^*_x\sin(2\phi) - \bar{\pi}^*_y\cos(2\phi)| \\
&= \frac{1}{\sqrt{2}}\left(|\pi^*_x,\bar{\pi}^*_x|\cos^2(2\phi) + |\pi^*_x,\bar{\pi}^*_y|\cos(2\phi)\sin(2\phi) + |\pi^*_y,\bar{\pi}^*_x|\cos(2\phi)\sin(2\phi) + |\pi^*_y,\bar{\pi}^*_y|\sin^2(2\phi)\right) \\
&+ \frac{1}{\sqrt{2}}\left(|\pi^*_x,\bar{\pi}^*_x|\sin^2(2\phi) - |\pi^*_x,\bar{\pi}^*_y|\cos(2\phi)\sin(2\phi) - |\pi^*_y,\bar{\pi}^*_x|\cos(2\phi)\sin(2\phi) + |\pi^*_y,\bar{\pi}^*_y|\cos^2(2\phi)\right) \\
&= \frac{1}{\sqrt{2}}\left(|\pi^*_x,\bar{\pi}^*_x| + |\pi^*_y,\bar{\pi}^*_y|\right) \\
&= \Psi
\end{aligned}
\tag{19}
$$

Hence $\Psi$ belongs to the represention with the character $+1$ for both $2C_\infty$ and $\infty\sigma_v$, i.e., $\Sigma_g^+$.

**Singlet Delta Oxygen (Normal Singlet Oxygen)** Normal ${}^1O_2$ is the ${}^1\Delta_g$ state. $\Delta_g$ is a doubly degenerate representation. That means that it has two components. These components are shown in the middle of Fig. 1 and should transform into linear combinations of each other under rotations and reflections. Let us check this.

Rotation:

$$
\begin{aligned}
\hat{R}(\phi)^1\Delta_g^{(1)} &= \frac{1}{\sqrt{2}}\left(|\pi^*_{x'},\bar{\pi}^*_{x'}| - |\bar{\pi}^*_{y'},\pi^*_{y'}|\right) \\
&= \frac{1}{\sqrt{2}}|\pi^*_x\cos\phi - \pi^*_y\sin\phi, \bar{\pi}^*_x\cos\phi - \bar{\pi}^*_y\sin\phi| \\
&- \frac{1}{\sqrt{2}}|\pi^*_x\sin\phi + \pi^*_y\cos\phi, \bar{\pi}^*_x\sin\phi + \bar{\pi}^*_y\cos\phi| \\
&= \frac{1}{\sqrt{2}}\left(|\pi^*_x,\bar{\pi}^*_x|\cos^2\phi - |\pi^*_x,\bar{\pi}^*_y|\cos\phi\sin\phi - |\pi^*_y,\bar{\pi}^*_x|\cos\phi\sin\phi + |\pi^*_y,\bar{\pi}^*_y|\sin^2\phi\right) \\
&- \frac{1}{\sqrt{2}}\left(|\pi^*_x,\bar{\pi}^*_x|\sin^2\phi - |\pi^*_x,\bar{\pi}^*_y|\cos\phi\sin\phi - |\pi^*_y,\bar{\pi}^*_x|\cos\phi\sin\phi - |\pi^*_y,\bar{\pi}^*_y|\cos^2\phi\right) \\
&= \frac{1}{\sqrt{2}}\left(|\pi^*_x,\bar{\pi}^*_x| - |\pi^*_y,\bar{\pi}^*_y|\right)\cos(2\phi) - \frac{1}{\sqrt{2}}\left(|\pi^*_x,\bar{\pi}^*_y| - |\bar{\pi}^*_x,\pi^*_y|\right)\sin(2\pi) \\
&= {}^1\Delta_g^{(1)}\cos(2\phi) -{}^1\,\Delta_g^{(2)}\sin(2\phi)
\end{aligned}
\tag{20}
$$

$$\begin{aligned}
\hat{R}(\phi)^1\Delta_g^{(2)} &= \frac{1}{\sqrt{2}}\left(|\pi^*_{x'},\bar{\pi}^*_{y'}| - |\bar{\pi}^*_{x'},\pi^*_{y'}|\right) \\
&= \frac{1}{\sqrt{2}}|\pi^*_x\cos\phi - \pi^*_y\sin\phi, \bar{\pi}^*_x\sin\phi + \bar{\pi}^*_y\cos\phi| \\
&- \frac{1}{\sqrt{2}}|\bar{\pi}^*_x\cos\phi - \bar{\pi}^*_y\sin\phi, \pi^*_x\sin\phi + \pi^*_y\cos\phi| \\
&= \frac{1}{\sqrt{2}}\left(|\pi^*_x,\bar{\pi}^*_x|\cos\phi\sin\phi + |\pi^*_x,\bar{\pi}^*_y|\cos^2\phi - |\pi^*_y,\bar{\pi}^*_x|\sin^2\phi - |\pi^*_y,\bar{\pi}^*_y|\cos\phi\sin\phi\right) \\
&- \frac{1}{\sqrt{2}}\left(|\bar{\pi}^*_x,\pi^*_x|\cos\phi\sin\phi + |\bar{\pi}^*_x,\pi^*_y|\cos^2\phi - |\bar{\pi}^*_y,\pi^*_x|\sin^2\phi - |\bar{\pi}^*_y,\pi^*_y|\cos\phi\sin\phi\right) \\
&= \frac{1}{\sqrt{2}}\left(|\pi^*_x,\bar{\pi}^*_x| - |\pi^*_y,\bar{\pi}^*_y|\right)\sin(2\phi) + \frac{1}{\sqrt{2}}\left(|\pi^*_x,\bar{\pi}^*_y| + |\bar{\pi}^*_x,\pi^*_y|\right)\cos(2\phi) \\
&= {}^1\Delta_g^{(1)}\sin(2\phi) +^1 \Delta_g^{(2)}\cos(2\phi) \qquad (21)
\end{aligned}$$

Hence

$$\hat{R}(\phi)\begin{pmatrix} {}^1\Delta_g^{(1)} & {}^1\Delta_g^{(2)} \end{pmatrix} = \begin{pmatrix} {}^1\Delta_g^{(1)} & {}^1\Delta_g^{(2)} \end{pmatrix}\begin{bmatrix} R_{1,1} & R_{1,2} \\ R_{2,1} & R_{2,2} \end{bmatrix} = \begin{pmatrix} {}^1\Delta_g^{(1)} & {}^1\Delta_g^{(2)} \end{pmatrix}\begin{bmatrix} \cos(2\phi) & \sin(2\phi) \\ -\sin(2\phi) & \cos(2\phi) \end{bmatrix} \qquad (22)$$

The character for the rotation is $\chi(R) = R_{1,1} + R_{2,2} = 2\cos(2\phi)$, in perfect agreement with the $\Delta_g$ character for $2C_\infty$.

Reflection:

$$\begin{aligned}
\hat{\sigma}_v(\phi)^1\Delta_g^{(1)} &= \frac{1}{\sqrt{2}}\left(|\pi^*_{x'},\bar{\pi}^*_{x'}| - |\bar{\pi}^*_{y'},\pi^*_{y'}|\right) \\
&= \frac{1}{\sqrt{2}}|\pi^*_x\cos(2\phi) + \pi^*_y\sin(2\phi), \bar{\pi}^*_x\cos(2\phi) + \bar{\pi}^*_y\sin(2\phi)| \\
&- \frac{1}{\sqrt{2}}|\pi^*_x\sin(2\phi) - \pi^*_y\cos(2\phi), \bar{\pi}^*_x\sin(2\phi) - \bar{\pi}^*_y\cos(2\phi)| \\
&= \frac{1}{\sqrt{2}}\left(|\pi^*_x,\bar{\pi}^*_x|\cos^2(2\phi) + |\pi^*_x,\bar{\pi}^*_y|\cos(2\phi)\sin(2\phi) + |\pi^*_y,\bar{\pi}^*_x|\cos(2\phi)\sin(2\phi) + |\pi^*_y,\bar{\pi}^*_y|\sin^2(2\phi)\right) \\
&- \frac{1}{\sqrt{2}}\left(|\pi^*_x,\bar{\pi}^*_x|\sin^2(2\phi) - |\pi^*_x,\bar{\pi}^*_y|\cos(2\phi)\sin(2\phi) - |\pi^*_y,\bar{\pi}^*_x|\cos(2\phi)\sin(2\phi) + |\pi^*_y,\bar{\pi}^*_y|\cos^2(2\phi)\right) \\
&= \frac{1}{\sqrt{2}}\left(|\pi^*_x,\bar{\pi}^*_x| - |\pi^*_y,\bar{\pi}^*_y|\right)\cos(4\phi) + \frac{1}{\sqrt{2}}\left(|\pi^*_x,\bar{\pi}^*_y| - |\bar{\pi}^*_x,\pi^*_y|\right)\sin(4\phi) \\
&= {}^1\Delta_g^{(1)}\cos(4\phi) +^1 \Delta_g^{(2)}\sin(4\phi) \qquad (23)
\end{aligned}$$

$$\begin{aligned}
\hat{\sigma}_v(\phi)^1\Delta_g^{(2)} &= \frac{1}{\sqrt{2}}\left(|\pi^*_{x'},\bar{\pi}^*_{y'}| - |\bar{\pi}^*_{x'},\pi^*_{y'}|\right) \\
&= \frac{1}{\sqrt{2}}||\pi^*_x\cos(2\phi) + \pi^*_y\sin(2\phi), \bar{\pi}^*_x\sin(2\phi) - \bar{\pi}^*_y\cos(2\phi)| \\
&- \frac{1}{\sqrt{2}}|\bar{\pi}^*_x\cos(2\phi) + \bar{\pi}^*_y\sin(2\phi), \pi^*_x\sin(2\phi) - \pi^*_y\cos(2\phi)| \\
&= \frac{1}{\sqrt{2}}\left(|\pi^*_x,\bar{\pi}^*_x|\cos(2\phi)\sin(2\phi) - |\pi^*_x,\bar{\pi}^*_y|\cos^2(2\phi) + |\pi^*_y,\bar{\pi}^*_x|\sin^2(2\phi) - |\pi^*_y,\bar{\pi}^*_y|\cos(2\phi)\sin(2\phi)\right) \\
&- \frac{1}{\sqrt{2}}\left(|\bar{\pi}^*_x,\pi^*_x|\cos(2\phi)\sin(2\phi) - |\bar{\pi}^*_x,\pi^*_y|\cos^2(2\phi) + |\bar{\pi}^*_y,\pi^*_x|\sin^2(2\phi) - |\bar{\pi}^*_y,\pi^*_y|\cos(2\phi)\sin(2\phi)\right) \\
&= \frac{1}{\sqrt{2}}\left(|\pi^*_x,\bar{\pi}^*_x| - |\pi^*_y,\bar{\pi}^*_y|\right)\sin(4\phi) - \frac{1}{\sqrt{2}}\left(|\pi^*_x,\bar{\pi}^*_y| - |\bar{\pi}^*_x,\pi^*_y|\right)\cos(4\phi) \\
&= {}^1\Delta_g^{(1)}\sin(4\phi) -^1 \Delta_g^{(2)}\cos(4\phi) \qquad (24)
\end{aligned}$$

Hence

$$\hat{\sigma}_v(\phi)\left(\begin{array}{cc} {}^1\Delta_g^{(1)} & {}^1\Delta_g^{(2)} \end{array}\right) = \left(\begin{array}{cc} {}^1\Delta_g^{(1)} & {}^1\Delta_g^{(2)} \end{array}\right)\left[\begin{array}{cc} \cos(4\phi) & \sin(4\phi) \\ \sin(4\phi) & -\cos(4\phi) \end{array}\right] \qquad (25)$$

and the corresponding character, which is the trace of the matrix, is zero in perfect agreement with the $\Delta_g$ character for $\infty\sigma_v$.

# 3 Sample deMon2k Input

The following is an example of a deMon2k input file for carrying out the $O_2$ MSM calculations reported here without any symmetry breaking.

```
TITLE O2
CHARGE 0
VXCTYPE BLYP
# ----- uncomment for step 1 ----------
# MULTI 1
# SCFTYPE UKS MAX=200
# SMEAR 0.05 UNIFORM
# ----- end step 1 commands--------------
# ----- uncomment for step 2a ------------
# MULTI 3
# SCFTYPE UKS MAX=0
# MOMODIFY 2 2
# 8 1
# 9 1
# 8 0
# 9 0
# ----- end step 2a commands--------------
# ----- uncomment for step 2b ------------
# MULTI 1
# SCFTYPE UKS MAX=0
# MOMODIFY 2 2
# 8 1
# 9 0
# 8 0
# 9 1
# ----- end step 2b commands--------------
# ----- uncomment for step 2c ------------
# MULTI 1
# SCFTYPE UKS MAX=0
# MOMODIFY 2 2
# 8 1
# 9 0
# 8 1
# 9 0
# ----- end step 2c commands--------------
#
PRINT MOS = 8-9
#
# --- GEOMETRY ---
#
#
GEOMETRY CARTESIAN BOHR
O 0.000000 0.000000 0.000000
```

```
O 0.000000 0.000000 3.100000
#
AUXIS (GEN-A3*)
BASIS (DEF2-TZVPP)
```

Lines beginning with a number sign (also called a hash mark or pound sign) are treated as comments and so are not part of the input. To do the calculation:

- First uncomment the block between "uncomment for step 1" and "end step 1 commands." This must be done before the other steps! Make sure it converges. It generates a restart file for the other calculations.
- Steps 2a, 2b, and 2c may be done in any order but we will give the instructions for doing them in alphabetical order. So recomment the step 1 block and uncomment the block between "uncomment for step 2a" and "end step 2a commands." This reads the orbitals from step 1 and changes the occupation to $\pi_x[\uparrow\ ][\uparrow\ ]\pi_y$ to do a calculation without any further self-consistent field (SCF) orbital relaxation calculations. The restart file is not modified. Just read the total energy at the end of the file.
- Recomment the step 2a block and uncomment the block between "uncomment for step 2b" and "end step 2b commands." This reads the orbitals from step 1 and changes the occupation to $\pi_x[\uparrow\ ][\ \downarrow]\pi_y$ to do a calculation without any further self-consistent field (SCF) orbital relaxation calculations. The restart file is not modified.
- Recomment the step 2b block and uncomment the block between "uncomment for step 2c" and "end step 2c commands." This reads the orbitals from step 1 and changes the occupation to $\pi_x[\uparrow\downarrow][\uparrow\downarrow]\pi_y$ to do a calculation without any further self-consistent field (SCF) orbital relaxation calculations. The restart file is not modified.

# 4 Multiplet sum method potential energy curves

**Figures 2**, **3**, **4**, **5**, **6**, **7**, **8**, and **9** show the graphs of the potential energy curves (PECs) obtained with different functionals using the multiplet sum method (MSM).

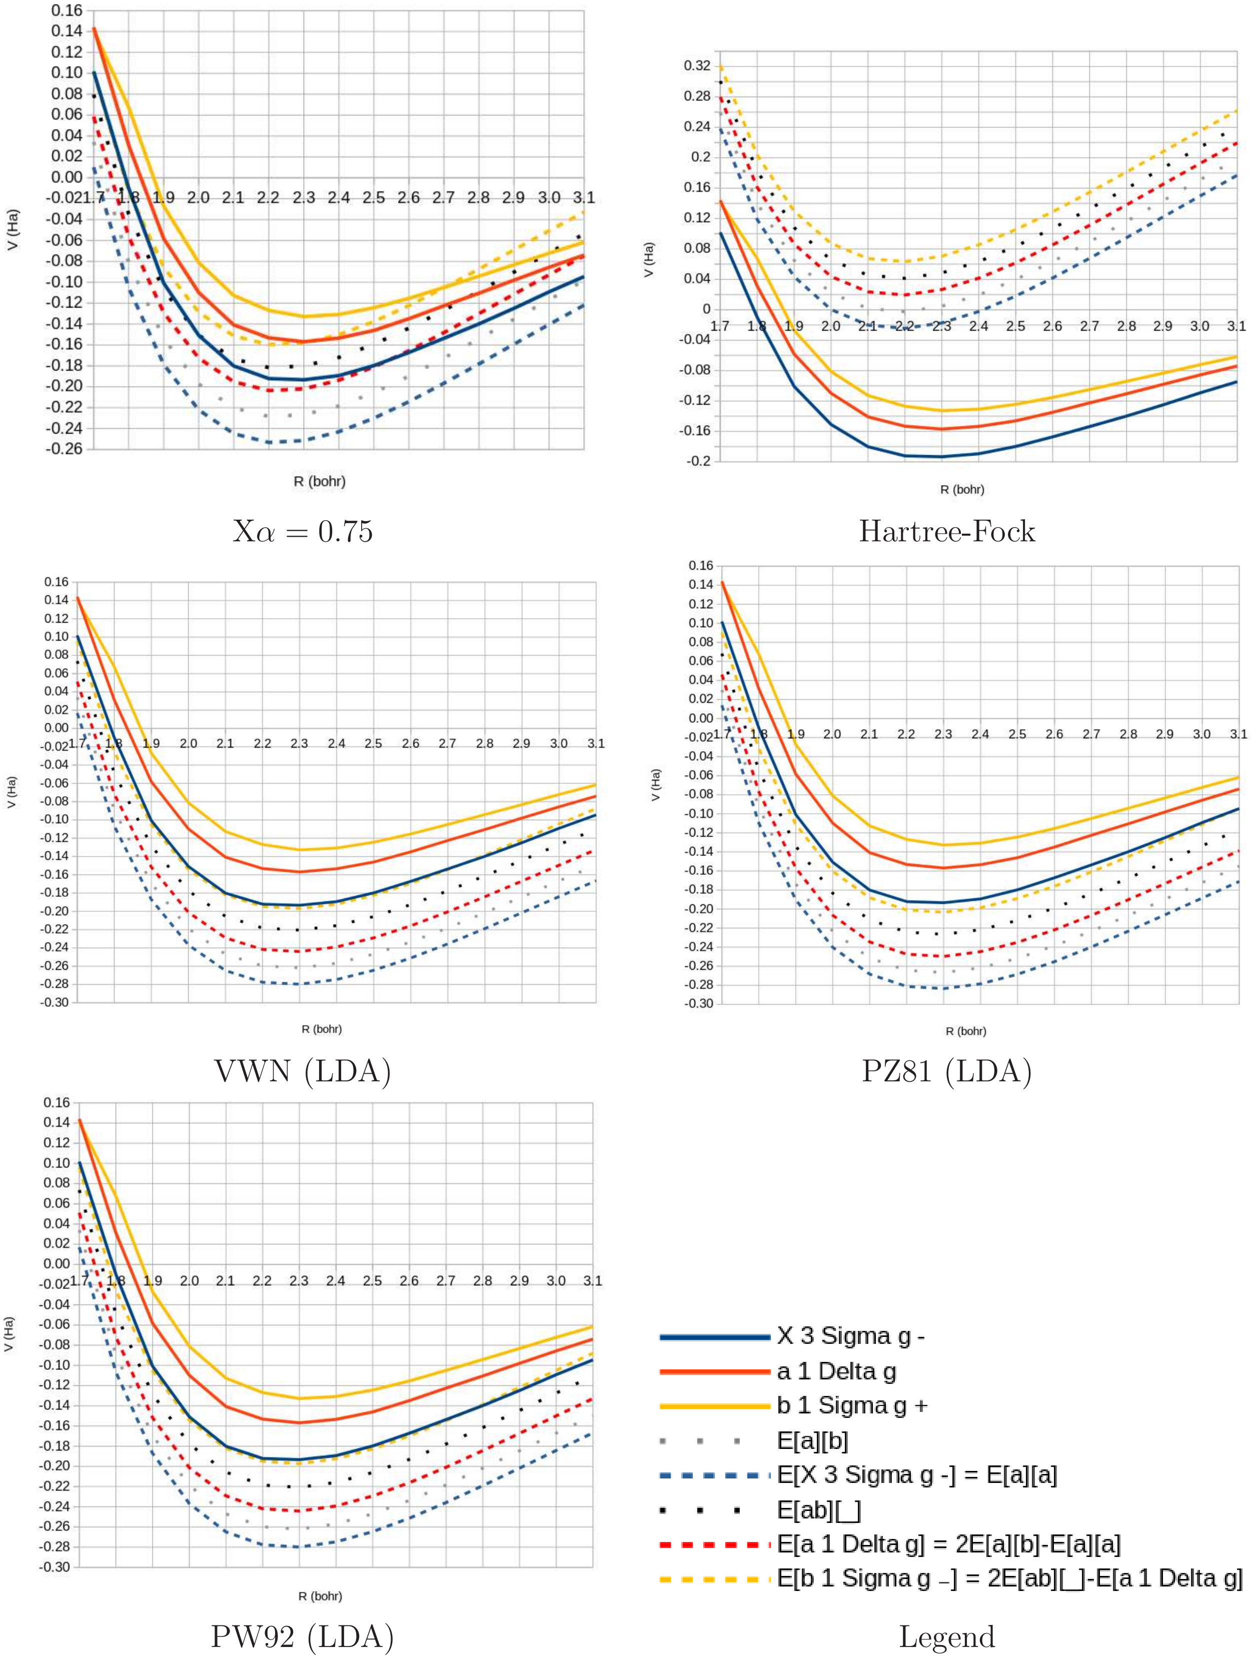


Figure 2: Comparison of MSM DFT $O_2$ PECs calculated with different functionals with reference curves.

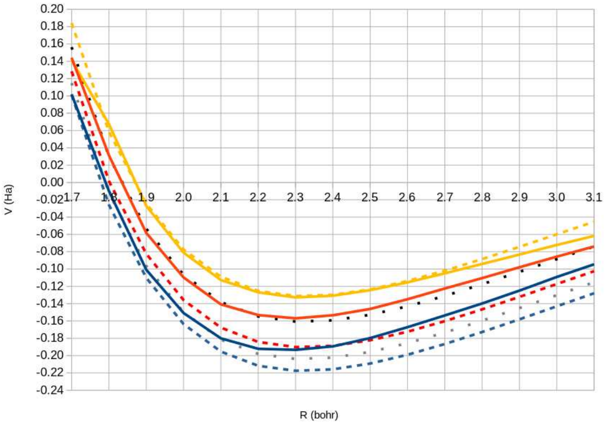


BLYP (GGA)

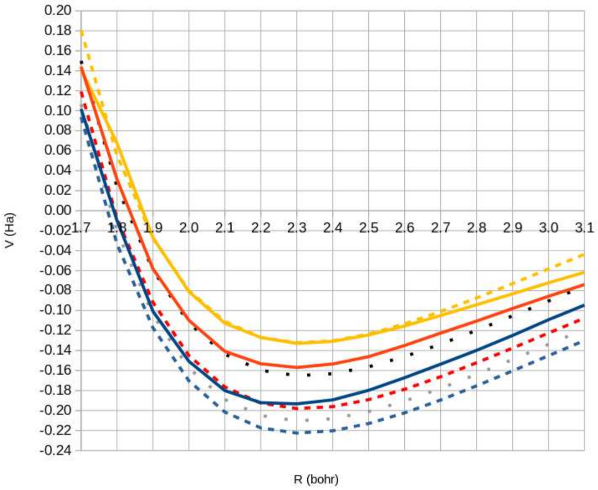


PW86 (GGA)

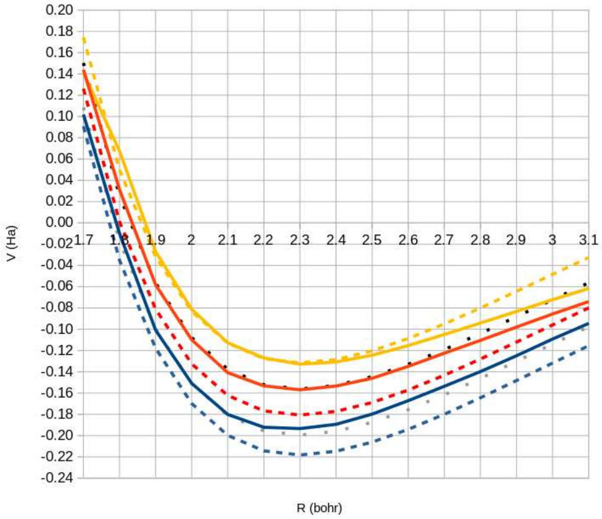


OLYP (GGA)

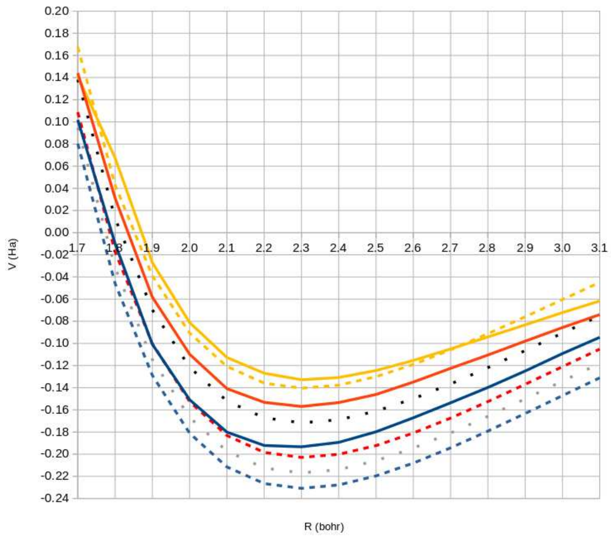


PW91 (GGA)

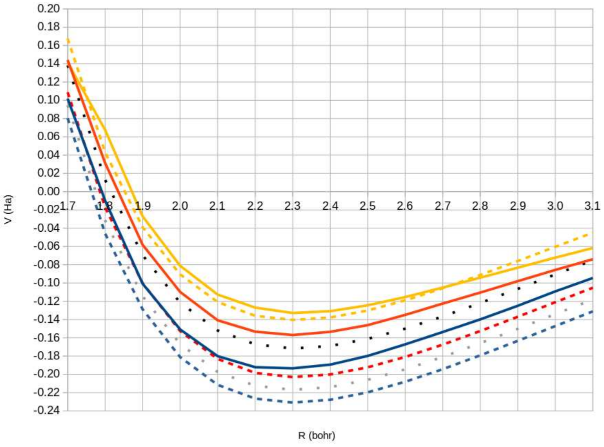


PW91SSF (GGA)

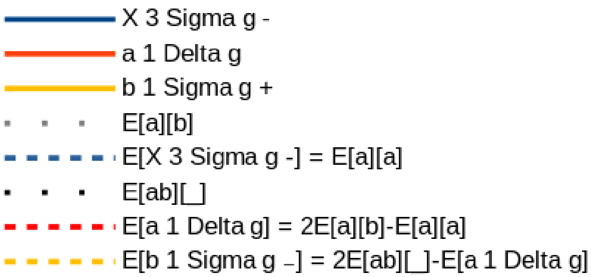


Legend

Figure 3: Comparison of MSM DFT $O_2$ PECs calculated with different functionals with reference curves.

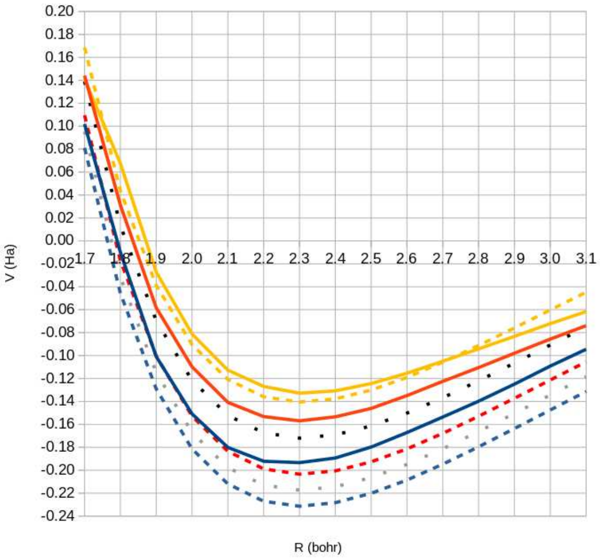


PBE (GGA)

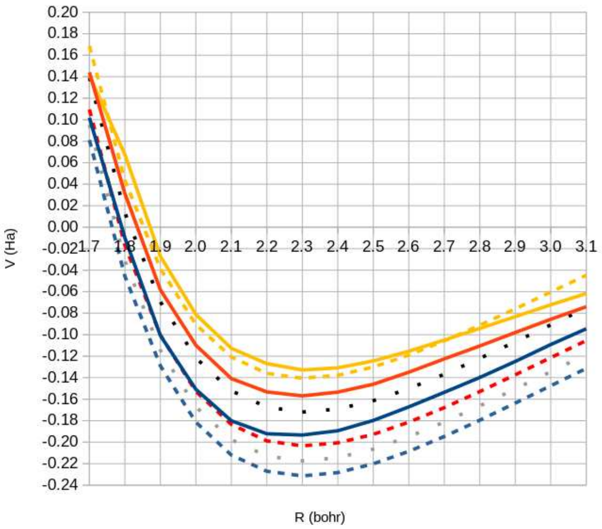


PBESSF (GGA)

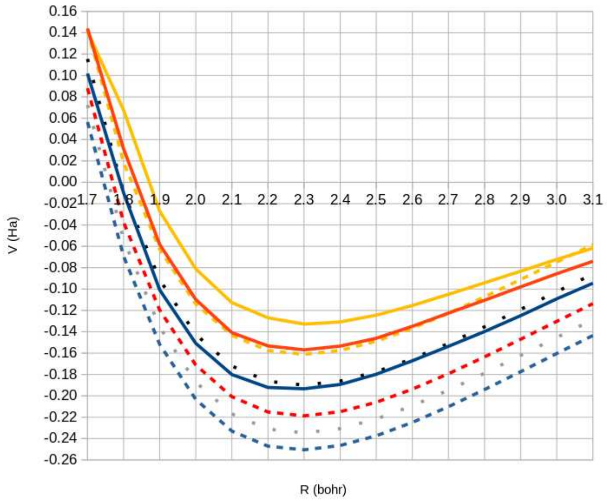


PBESOL (GGA)

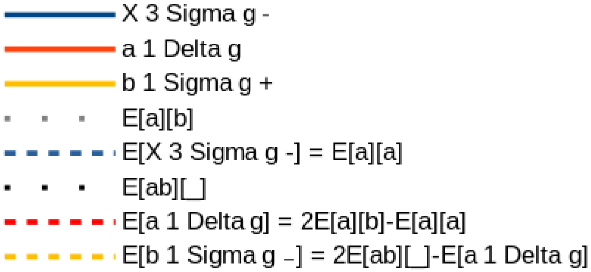


Legend

Figure 4: Comparison of MSM DFT $O_2$ PECs calculated with different functionals with reference curves.

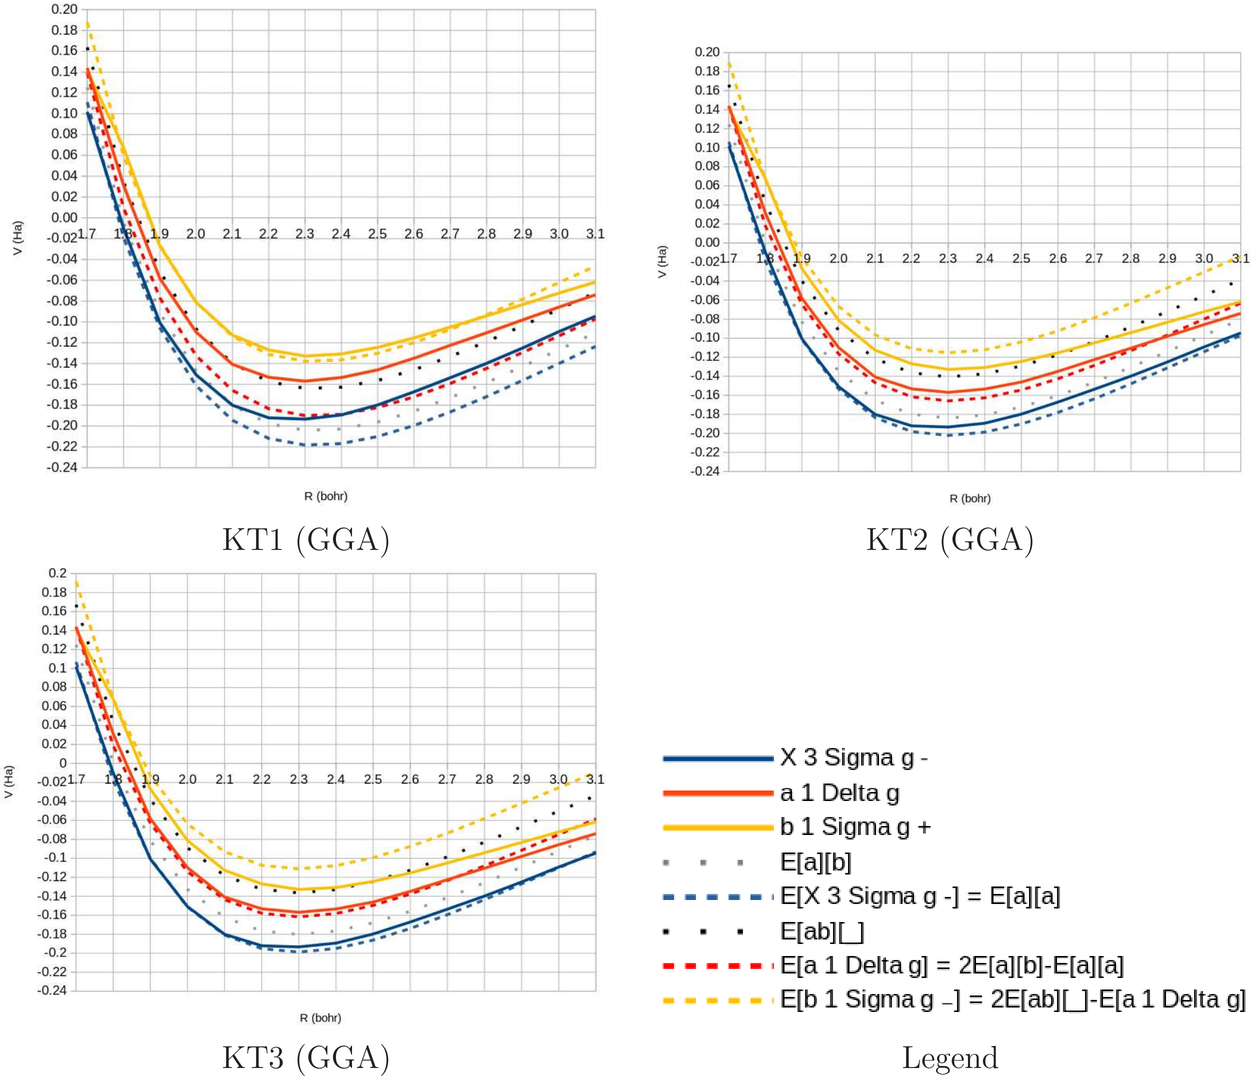


Figure 5: Comparison of MSM DFT $O_2$ PECs calculated with different functionals with reference curves.

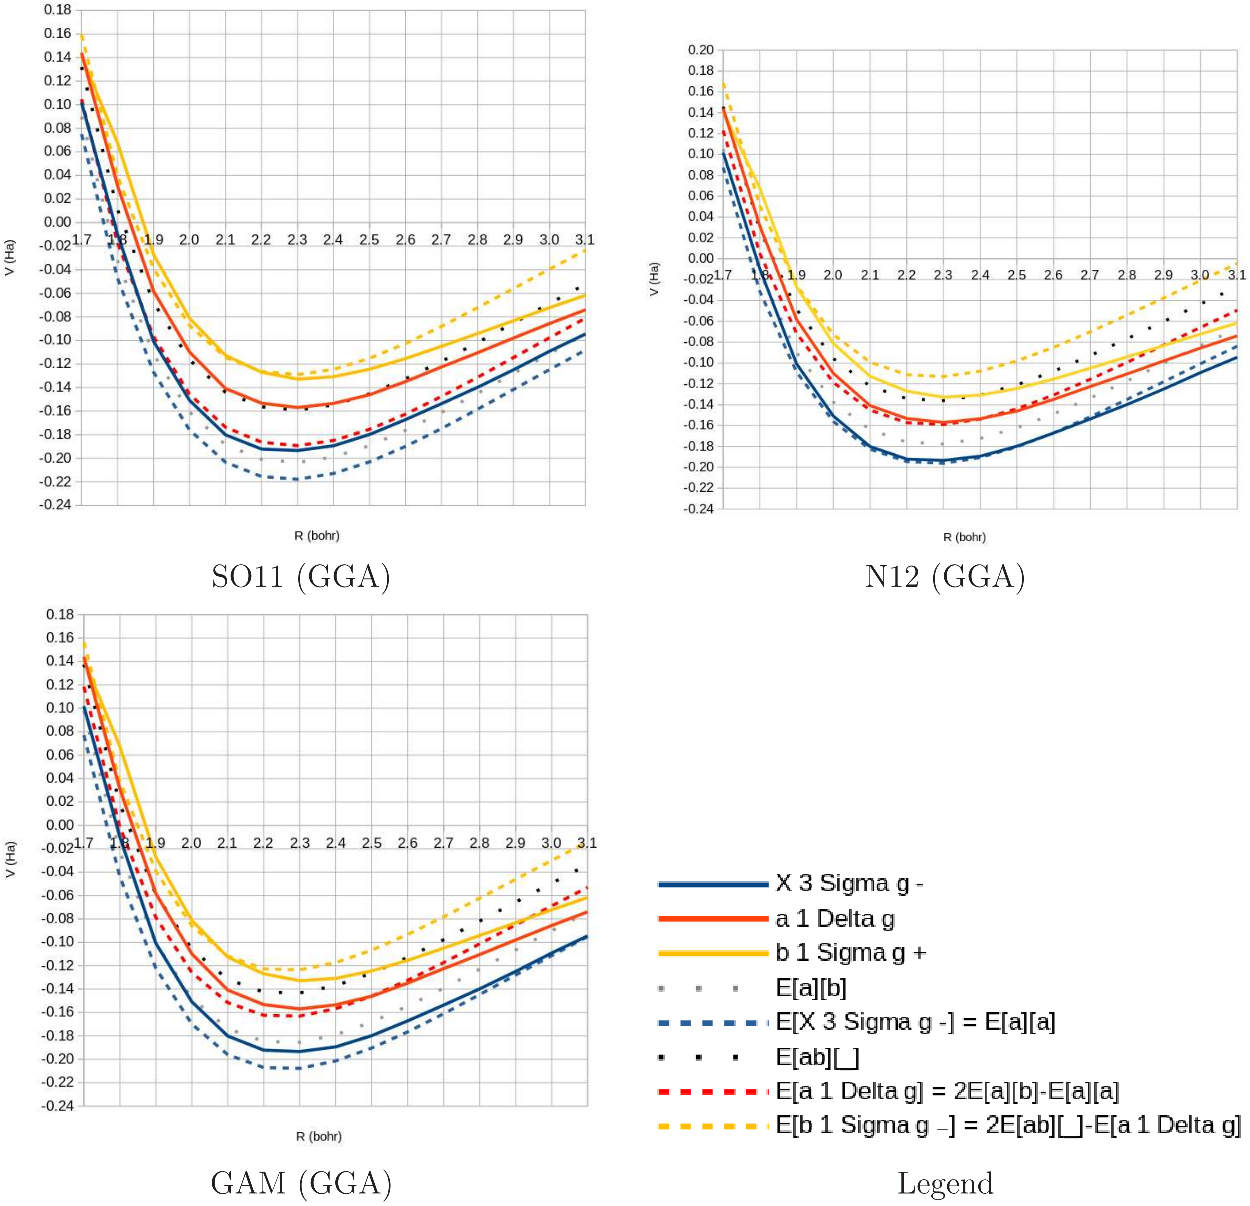


Figure 6: Comparison of MSM DFT $O_2$ PECs calculated with different functionals with reference curves.

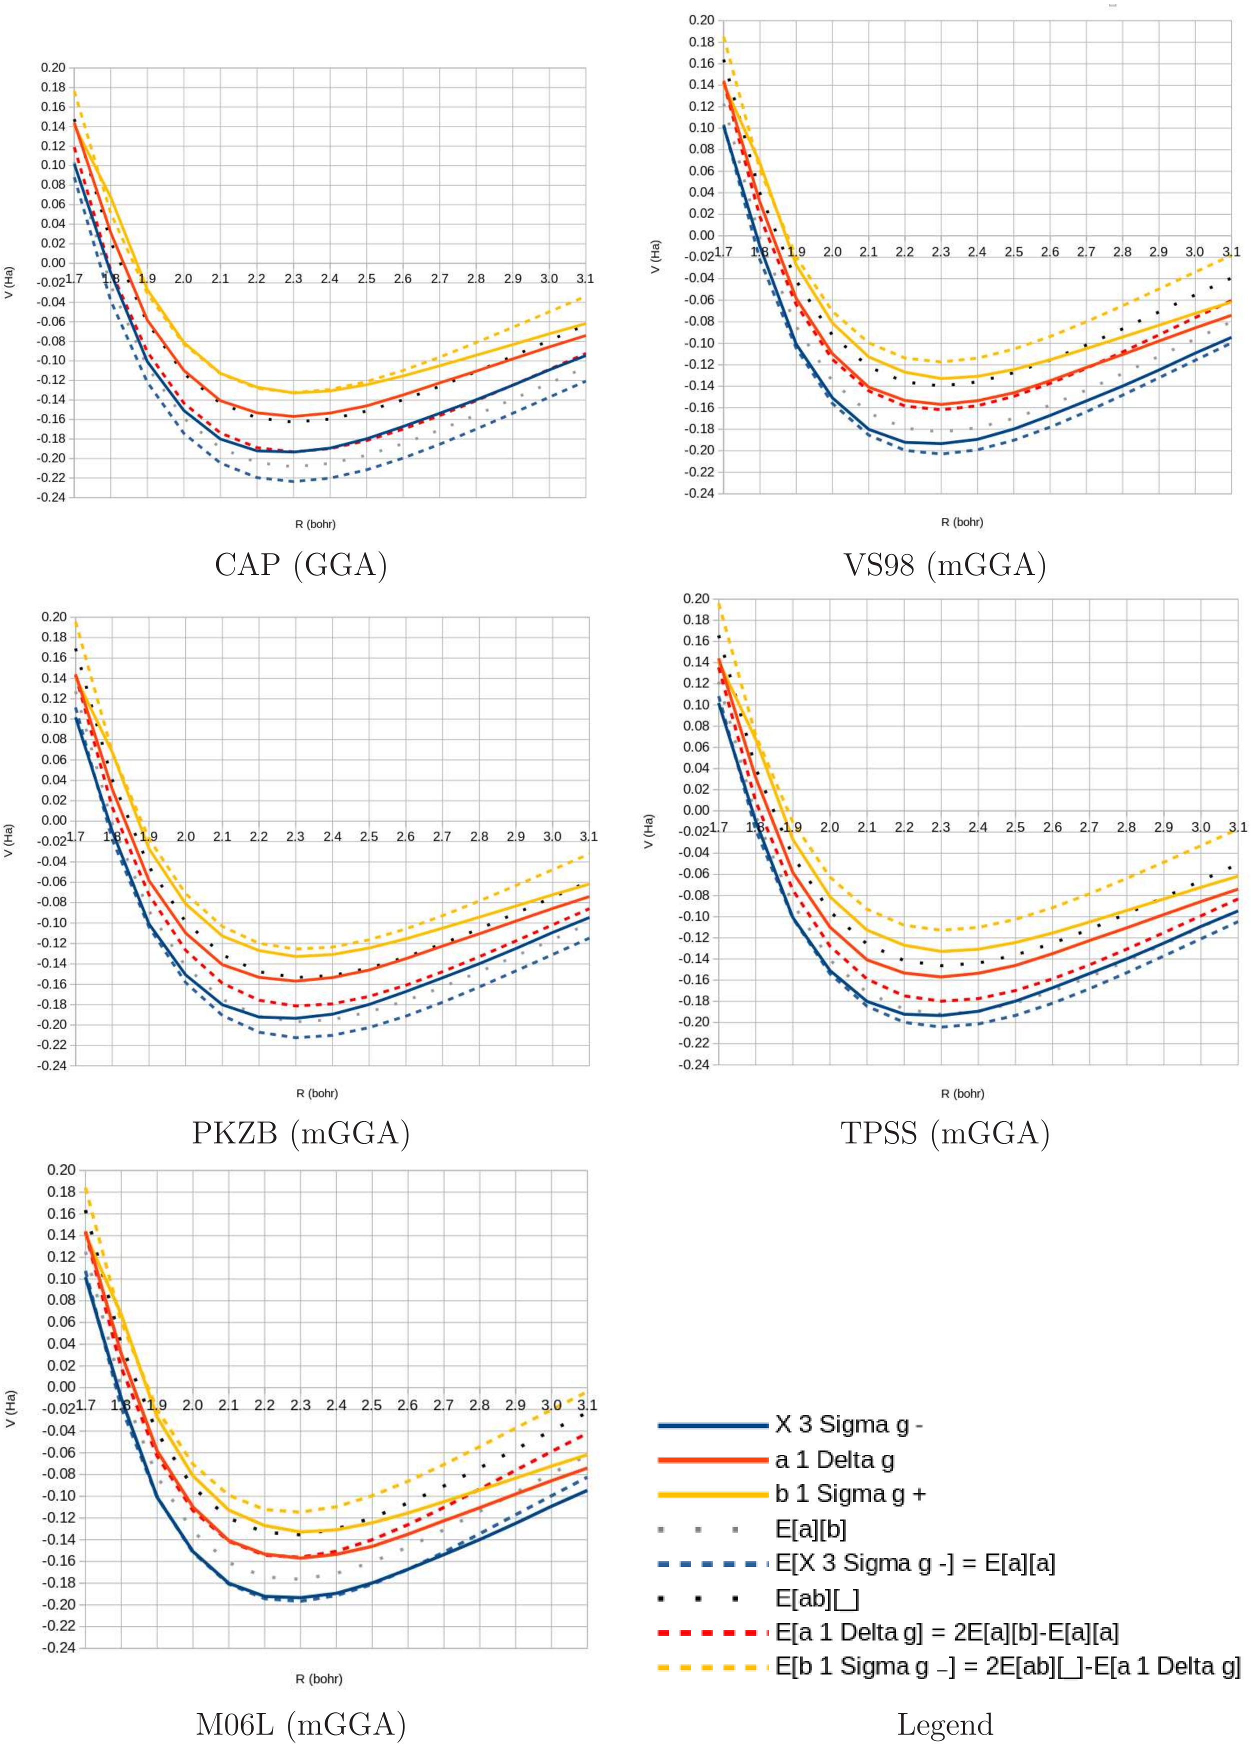


Figure 7: Comparison of MSM DFT $O_2$ PECs calculated with different functionals with reference curves.

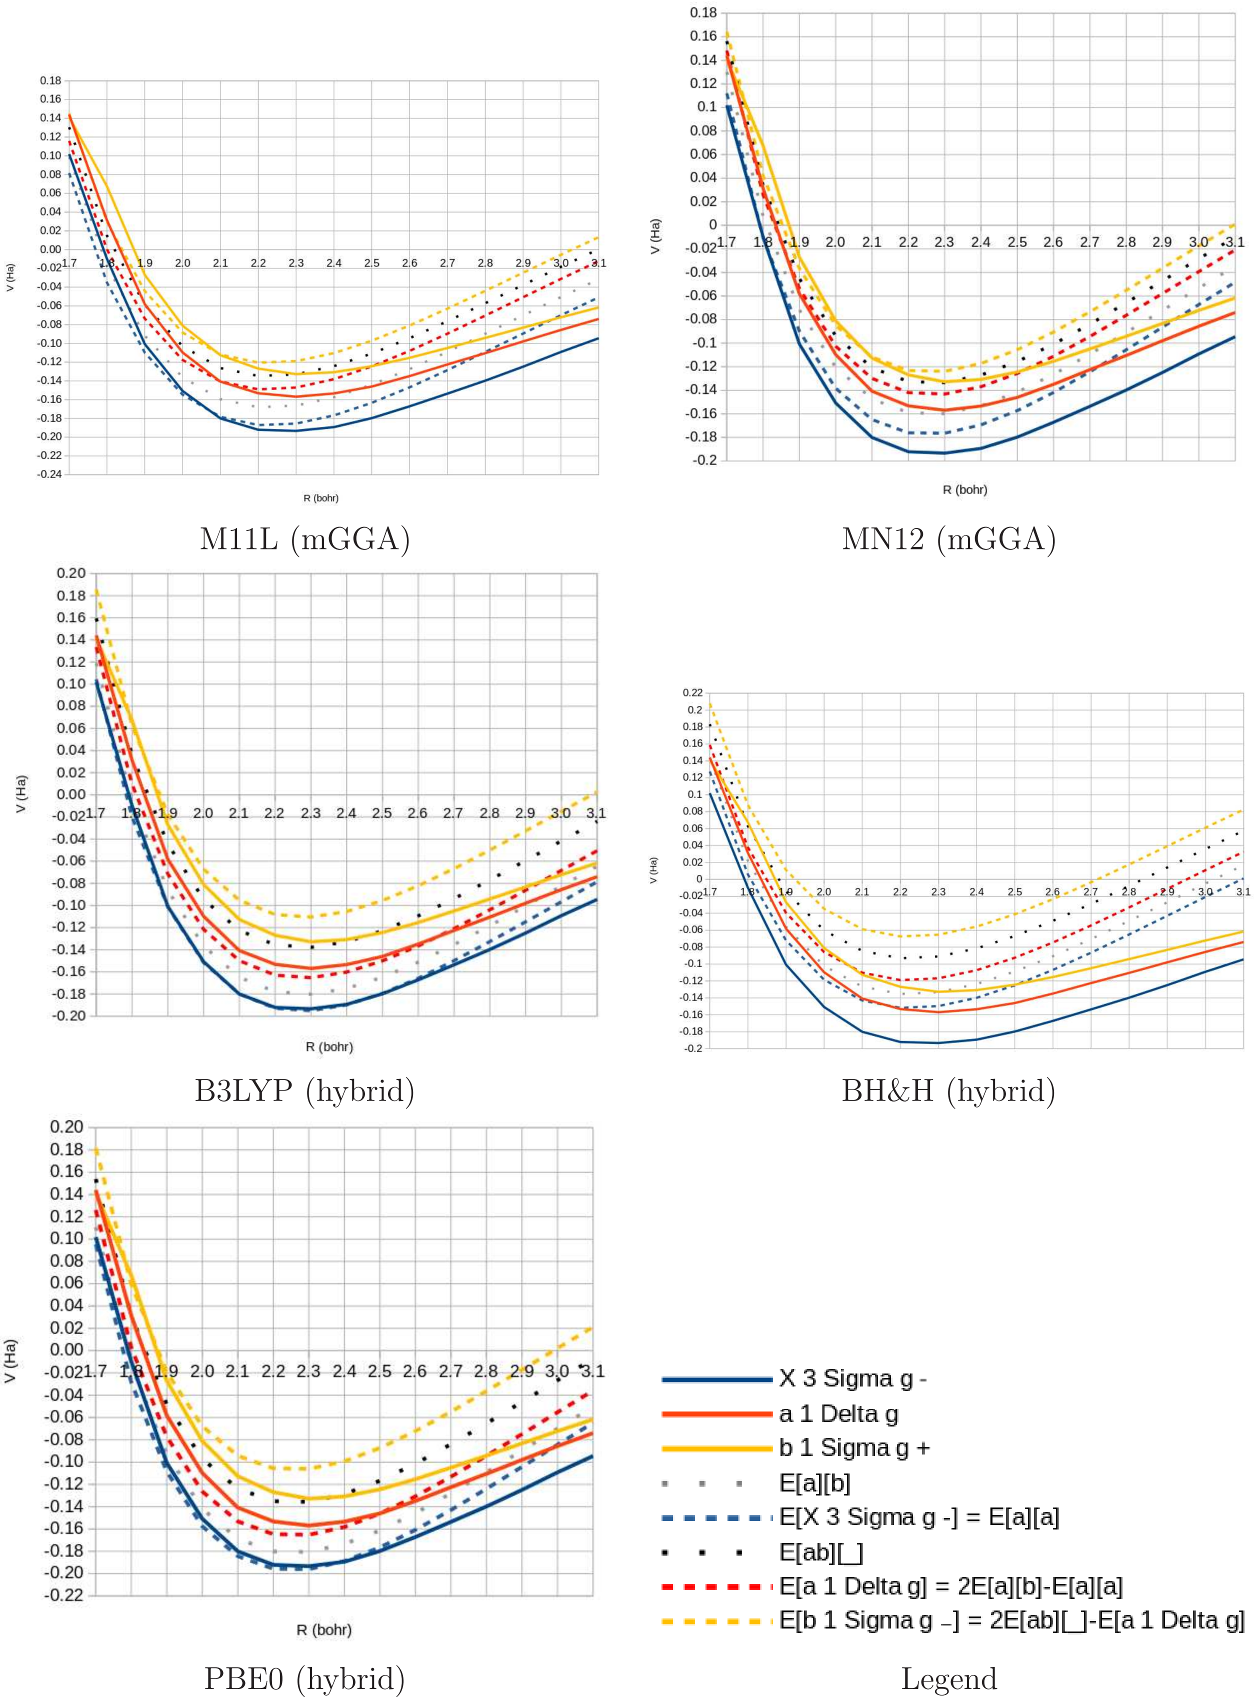


Figure 8: Comparison of MSM DFT $O_2$ PECs calculated with different functionals with reference curves.

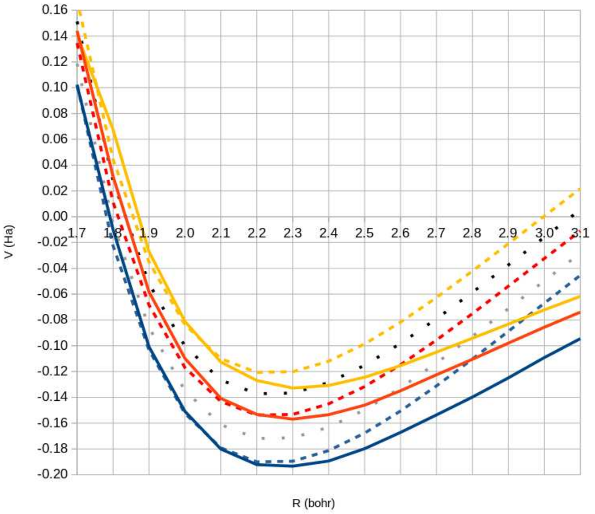


M062X (mGGA hybrid)

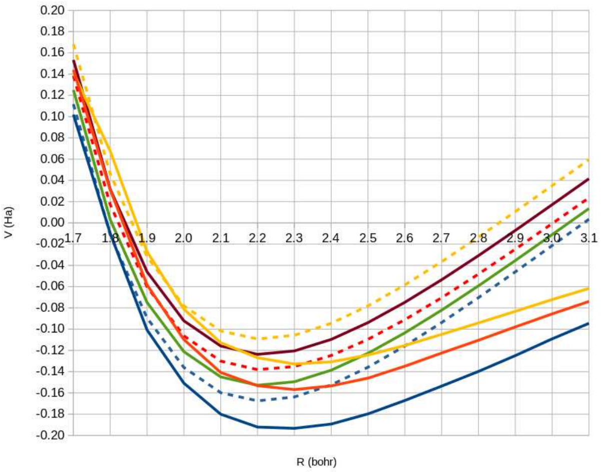


M06HF (mGGA hybrid)

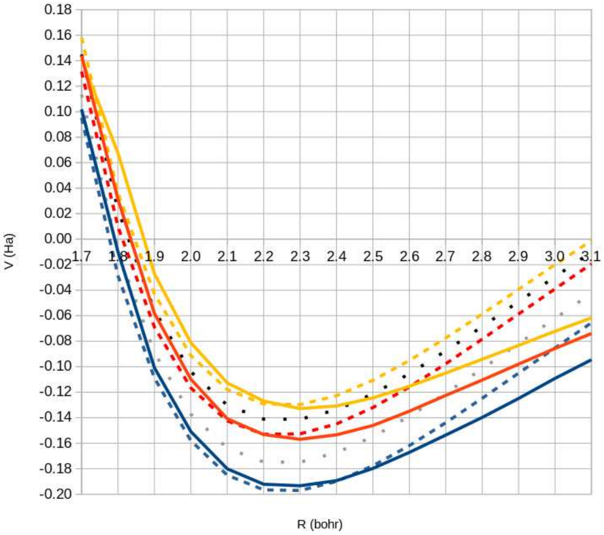


M06 (mGGA hybrid)

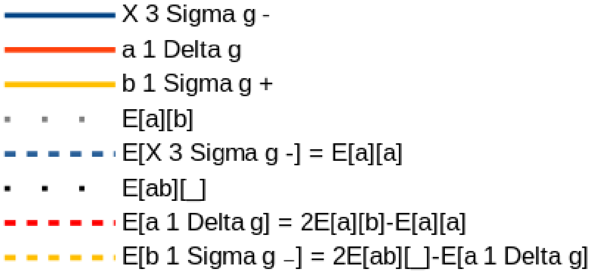


Legend

Figure 9: Comparison of MSM DFT $O_2$ PECs calculated with different functionals with reference curves.

# 5 Tables comparing calculated and experimental atomic and diatomic calculated parameters

This section provides numerical tables which are the basis for graphs presented in the main text.

Atomic energies are given in **Table 3**. In this and other tables, extensive references are given to orginal papers treating each functional. References are also give to our sources of best estimate comparison data.

Binding energies are given in **Table 4**.

Vertical and adiabatic excitation energies are given in **Table 5**.

Bond distances are given in **Table 6**.

Harmonic frequencies are given in **Table 7** and anharmonic corrections (calculated using the Morse formula) are given in **Table 8**.

Table 3: Total nonrelativistic energy of the ground state oxygen atom as calculated with different functionals and the DEF2-TZVPP basis set. (1 Ha = 627.5 kcal/mol = 27.2114 eV.)

| Functional | Energy (Ha) |
|---|---|
| X$\alpha$ = 0.75 [3] | -74.910368906 |
| Hartree-Fock [4] | -74.815596473 |
| VWN (LDA) [5, 6] | -74.523841645 |
| PZ81 (LDA) [5, 7] | -74.516424670 |
| PW92 (LDA) [5, 8] | -74.521199538 |
| BLYP (GGA) [9, 10, 11] | -75.082982384 |
| PW86 (GGA) [12, 13] | -75.157433340 |
| OLYP (GGA) [10, 14, 11] | -75.072518435 |
| PW91 (GGA) [15] | -75.060596371 |
| PW91SSF (GGA) [15] | -75.060596363 |
| PBE (GGA) [16, 17] | -75.007287689 |
| PBESSF (GGA) [16, 17] | -75.007287495 |
| PBESOL (GGA) [18, 19] | -74.752792437 |
| KT1 (GGA) [20, 21] | -76.010267736 |
| KT2 (GGA) [20, 21] | -76.161101302 |
| KT3 (GGA) [20, 21] | -76.070104788 |
| SO11 (GGA) [22] | -75.076931764 |
| N12 (GGA) [23] | -75.064292317 |
| GAM (GGA) [24] | -75.066959927 |
| CAP (GGA) [25] | -74.913085710 |
| VS98 (mGGA) [26, 27] | -75.111416632 |
| PKZB (mGGA) [28, 29] | -74.959485696 |
| TPSS (mGGA) [30, 31] | -75.102039604 |
| M06L (mGGA) [32] | -75.083281979 |
| M11L (mGGA) [33] | -75.063902707 |
| MN12 (mGGA) [34] | -75.032008853 |
| B3LYP (hybrid) [35, 36] | -75.094004392 |
| BH&H (hybrid) [37] | -75.074365025 |
| PBE0 (hybrid) [38, 39] | -75.015995415 |
| M062X (mGGA hybrid) [40] | -75.063077144 |
| M06HF (mGGA hybrid) [40] | -75.071831377 |
| M06 (mGGA hybrid) [40] | -75.055319249 |
| Best Estimate [41] | -75.0673 |

Table 4: $O_2$ bond energy (Ha) calculated with different functionals and the DEF2-TZVPP basis set. (1 Ha = 627.5 kcal/mol.)

| Functional | $X\,^1\Sigma_g^-$ | $a\,^1\Delta_g$ | $b\,^1\Sigma_g^+$ |
|---|---|---|---|
| X$\alpha$ = 0.75 [3] | 0.25380 | 0.20419 | 0.16030 |
| Hartree-Fock [4] | 0.02445 | -0.01938 | -0.06320 |
| VWN (LDA) [5, 6] | 0.27987 | 0.24411 | 0.19715 |
| PZ81 (LDA) [5, 7] | 0.28367 | 0.24983 | 0.20345 |
| PW92 (LDA) [5, 8] | 0.28001 | 0.24437 | 0.19741 |
| BLYP (GGA) [9, 10, 11] | 0.21782 | 0.19054 | 0.13152 |
| PW86 (GGA) [12, 13] | 0.22268 | 0.19825 | 0.13237 |
| OLYP (GGA) [10, 14, 11] | 0.21821 | 0.18064 | 0.13169 |
| PW91 (GGA) [15] | 0.23088 | 0.20300 | 0.14049 |
| PW91SSF (GGA) [15] | 0.23088 | 0.20300 | 0.14049 |
| PBE (GGA) [16, 17] | 0.23142 | 0.20347 | 0.14058 |
| PBESSF (GGA) [16, 17] | 0.23142 | 0.20347 | 0.14058 |
| PBSOL (GGA) [18, 19] | 0.25056 | 0.21872 | 0.16119 |
| KT1 (GGA) [20, 21] | 0.21869 | 0.19046 | 0.13820 |
| KT2 (GGA) [20, 21] | 0.20216 | 0.16588 | 0.11534 |
| KT3 (GGA) [20, 21] | 0.19878 | 0.16170 | 0.11117 |
| SO11 (GGA) [22] | 0.21790 | 0.18927 | 0.12906 |
| N12 (GGA) [23] | 0.19649 | 0.15927 | 0.11322 |
| GAM (GGA) [24] | 0.20832 | 0.16359 | 0.12398 |
| CAP (GGA) [25] | 0.22358 | 0.19315 | 0.13237 |
| VS98 (mGGA) [26, 27] | 0.20305 | 0.16190 | 0.11743 |
| PKZB (mGGA) [28, 29] | 0.21257 | 0.18150 | 0.12568 |
| TPSS (mGGA) [30, 31] | 0.20433 | 0.17996 | 0.11284 |
| M06L (mGGA) [32] | 0.19673 | 0.15638 | 0.11471 |
| M11L (mGGA) [33] | 0.18778 | 0.14857 | 0.12113 |
| MN12 (mGGA) [34] | 0.17720 | 0.14363 | 0.12453 |
| B3LYP (hybrid) [35, 36] | 0.19522 | 0.16541 | 0.11058 |
| BH&H (hybrid) [37] | 0.15234 | 0.11948 | 0.06791 |
| PBE0 (hybrid) [38, 39] | 0.19674 | 0.16584 | 0.10676 |
| M062X (mGGA hybrid) [40] | 0.19116 | 0.15488 | 0.12178 |
| M06HF (mGGA hybrid) [40] | 0.16766 | 0.13844 | 0.10951 |
| M06 (mGGA hybrid) [40] | 0.19778 | 0.15417 | 0.13042 |
| Best Estimate [1] | 0.19354 | 0.15692 | 0.13306 |

Table 5: $O_2$ excitation energies (Ha) calculated with different functionals and the DEF2-TZVPP basis set. (1 Ha = 27.2114 eV.) Note that there is some numerical uncertainty (roughly ±1) in the last digit.

| Functional | Vertical | | Adiabatic | |
|---|---|---|---|---|
| | $a\,^1\Delta_g$ | $b\,^1\Sigma_g^+$ | $a\,^1\Delta_g$ | $b\,^1\Sigma_g^+$ |
| Functional | $X\,^1\Sigma_g^-$ | $a\,^1\Delta_g$ | $b\,^1\Sigma_g^+$ | |
| X$\alpha = 0.75$ [3] | 0.04961 | 0.09349 | 0.04961 | 0.09350 |
| Hartree-Fock [4] | 0.04383 | 0.08765 | 0.04383 | 0.08765 |
| VWN (LDA) [5, 6] | 0.03576 | 0.08271 | 0.03576 | 0.08272 |
| PZ81 (LDA) [5, 7] | 0.03383 | 0.08021 | 0.03384 | 0.08022 |
| PW92 (LDA) [5, 8] | 0.03563 | 0.08259 | 0.03564 | 0.08260 |
| BLYP (GGA) [9, 10, 11] | 0.02727 | 0.08628 | 0.02728 | 0.08630 |
| PW86 (GGA) [12, 13] | 0.02444 | 0.09031 | 0.02443 | 0.09031 |
| OLYP (GGA) [10, 14, 11] | 0.03757 | 0.08653 | 0.03757 | 0.08652 |
| PW91 (GGA) [15] | 0.02788 | 0.09039 | 0.02788 | 0.09039 |
| PW91SSF (GGA) [15] | 0.02788 | 0.09039 | 0.02788 | 0.09039 |
| PBE (GGA) [16, 17] | 0.02795 | 0.09083 | 0.02795 | 0.09084 |
| PBESSF (GGA) [16, 17] | 0.02795 | 0.09083 | 0.02795 | 0.09084 |
| PBESOL (GGA) [18, 19] | 0.03183 | 0.08937 | 0.03184 | 0.08937 |
| KT1 (GGA) [20, 21] | 0.02823 | 0.08048 | 0.02823 | 0.08049 |
| KT2 (GGA) [20, 21] | 0.03626 | 0.08680 | 0.03628 | 0.08682 |
| KT3 (GGA) [20, 21] | 0.03707 | 0.08762 | 0.03708 | 0.08761 |
| SO11 (GGA) [22] | 0.02861 | 0.08882 | 0.02863 | 0.08884 |
| N12 (GGA) [23] | 0.03721 | 0.08325 | 0.03722 | 0.08327 |
| GAM (GGA) [24] | 0.04471 | 0.08433 | 0.04473 | 0.08434 |
| CAP (GGA) [25] | 0.03041 | 0.09118 | 0.03043 | 0.09121 |
| VS98 (mGGA) [26, 27] | 0.04115 | 0.08562 | 0.04115 | 0.08562 |
| PKZB (mGGA) [28, 29] | 0.03107 | 0.08689 | 0.03107 | 0.08689 |
| TPSS (mGGA) [30, 31] | 0.02440 | 0.09149 | 0.02437 | 0.09149 |
| M06L (mGGA) [32] | 0.04034 | 0.08200 | 0.04035 | 0.08202 |
| M11L (mGGA) [33] | 0.03819 | 0.06663 | 0.03821 | 0.06665 |
| MN12 (mGGA) [34] | 0.03367 | 0.05270 | 0.03357 | 0.05267 |
| B3LYP (hybrid) [35, 36] | 0.02981 | 0.08463 | 0.02981 | 0.08464 |
| BH&H (hybrid) [37] | 0.03285 | 0.08440 | 0.03286 | 0.08443 |
| PBE0 (hybrid) [38, 39] | 0.03090 | 0.08997 | 0.03090 | 0.08998 |
| M062X (mGGA hybrid) [40] | 0.03626 | 0.06936 | 0.03628 | 0.06938 |
| M06HF (mGGA hybrid) [40] | 0.02920 | 0.05815 | 0.02922 | 0.05815 |
| M06 (mGGA hybrid) [40] | 0.04408 | 0.06735 | 0.04361 | 0.06736 |
| Best Estimate [1] | 0.03718 | 0.07017 | 0.03607 | 0.06577 |
| Best Estimate [42] | | | 0.0360775 | 0.0601213 |

Table 6: $O_2$ bond distance (bohr) calculated with different functionals and the DEF2-TZVPP basis set. (1 bohr = 0.5292 Å.)

| Functional | $X\,^1\Sigma_g^-$ | $a\,^1\Delta_g$ | $b\,^1\Sigma_g^+$ |
|---|---|---|---|
| X$\alpha$ = 0.75 [3] | 2.23 | 2.23 | 2.24 |
| Hartree-Fock [4] | 2.19 | 2.19 | 2.19 |
| VWN (LDA) [5, 6] | 2.28 | 2.28 | 2.28 |
| PZ81 (LDA) [5, 7] | 2.28 | 2.28 | 2.28 |
| PW92 (LDA) [5, 8] | 2.28 | 2.28 | 2.28 |
| BLYP (GGA) [9, 10, 11] | 2.33 | 2.33 | 2.33 |
| PW86 (GGA) [12, 13] | 2.32 | 2.32 | 2.32 |
| OLYP (GGA) [10, 14, 11] | 2.30 | 2.30 | 2.31 |
| PW91 (GGA) [15] | 2.31 | 2.31 | 2.31 |
| PW91SSF (GGA) [15] | 2.31 | 2.31 | 2.31 |
| PBE (GGA) [16, 17] | 2.31 | 2.31 | 2.31 |
| PBESSF (GGA) [16, 17] | 2.31 | 2.31 | 2.31 |
| PBSOL (GGA) [18, 19] | 2.30 | 2.30 | 2.30 |
| KT1 (GGA) [20, 21] | 2.33 | 2.33 | 2.33 |
| KT2 (GGA) [20, 21] | 2.30 | 2.31 | 2.31 |
| KT3 (GGA) [20, 21] | 2.30 | 2.30 | 2.30 |
| SO11 (GGA) [22] | 2.28 | 2.29 | 2.29 |
| N12 (GGA) [23] | 2.27 | 2.28 | 2.28 |
| GAM (GGA) [24] | 2.26 | 2.26 | 2.26 |
| CAP (GGA) [25] | 2.30 | 2.31 | 2.31 |
| VS98 (mGGA) [26, 27] | 2.30 | 2.30 | 2.30 |
| PKZB (mGGA) [28, 29] | 2.32 | 2.32 | 2.32 |
| TPSS (mGGA) [30, 31] | 2.31 | 2.32 | 2.31 |
| M06L (mGGA) [32] | 2.28 | 2.28 | 2.28 |
| M11L (mGGA) [33] | 2.23 | 2.23 | 2.23 |
| MN12 (mGGA) [34] | 2.25 | 2.27 | 2.26 |
| B3LYP (hybrid) [35, 36] | 2.28 | 2.28 | 2.28 |
| BH&H (hybrid) [37] | 2.23 | 2.23 | 2.23 |
| PBE0 (hybrid) [38, 39] | 2.25 | 2.26 | 2.26 |
| M062X (mGGA hybrid) [40] | 2.25 | 2.25 | 2.25 |
| M06HF (mGGA hybrid) [40] | 2.22 | 2.22 | 2.22 |
| M06 (mGGA hybrid) [40] | 2.26 | 2.25 | 2.26 |
| Best Estimate [1] | 2.27 | 2.30 | 2.32 |
| Best Estimate [42] | 2.28 | 2.30 | 2.32 |

Table 7: $O_2$ harmonic vibrational ($omega_e$) frequencies (Ha) calculated with different functionals and the DEF2-TZVPP basis set. (1 Ha = 219474.6 $cm^{-1}$.)

| Functional | $X\,^1\Sigma_g^-$ | $a\,^1\Delta_g$ | $b\,^1\Sigma_g^+$ |
|---|---|---|---|
| X$\alpha = 0.75$ [3] | 0.008278 | 0.008239 | 0.008205 |
| Hartree-Fock [4] | 0.008826 | 0.008787 | 0.008748 |
| VWN (LDA) [5, 6] | 0.007078 | 0.007048 | 0.007012 |
| PZ81 (LDA) [5, 7] | 0.007082 | 0.007051 | 0.007014 |
| PW92 (LDA) [5, 8] | 0.007079 | 0.007049 | 0.007013 |
| BLYP (GGA) [9, 10, 11] | 0.007114 | 0.007103 | 0.007049 |
| PW86 (GGA) [12, 13] | 0.007117 | 0.007102 | 0.007052 |
| OLYP (GGA) [10, 14, 11] | 0.007120 | 0.007073 | 0.007055 |
| PW91 (GGA) [15] | 0.007125 | 0.007117 | 0.007059 |
| PW91SSF (GGA) [15] | 0.007125 | 0.007117 | 0.007059 |
| PBE (GGA) [16, 17] | 0.007140 | 0.007133 | 0.007072 |
| PBESSF (GGA) [16, 17] | 0.007140 | 0.007133 | 0.007072 |
| PBSOL (GGA) [18, 19] | 0.007146 | 0.007128 | 0.007079 |
| KT1 (GGA) [20, 21] | 0.007292 | 0.007280 | 0.007228 |
| KT2 (GGA) [20, 21] | 0.007139 | 0.007125 | 0.007076 |
| KT3 (GGA) [20, 21] | 0.007104 | 0.007073 | 0.007043 |
| SO11 (GGA) [22] | 0.007055 | 0.007090 | 0.006999 |
| N12 (GGA) [23] | 0.006993 | 0.006969 | 0.006936 |
| GAM (GGA) [24] | 0.006947 | 0.006872 | 0.006876 |
| CAP (GGA) [25] | 0.007167 | 0.007162 | 0.007102 |
| VS98 (mGGA) [26, 27] | 0.007104 | 0.007070 | 0.007035 |
| PKZB (mGGA) [28, 29] | 0.007277 | 0.007261 | 0.007214 |
| TPSS (mGGA) [30, 31] | 0.007152 | 0.007166 | 0.007079 |
| M06L (mGGA) [32] | 0.007230 | 0.007172 | 0.007153 |
| M11L (mGGA) [33] | 0.006976 | 0.006923 | 0.007126 |
| MN12 (mGGA) [34] | 0.007142 | 0.007779 | 0.007126 |
| B3LYP (hybrid) [35, 36] | 0.007143 | 0.007122 | 0.007068 |
| BH&H (hybrid) [37] | 0.008657 | 0.008629 | 0.008583 |
| PBE0 (hybrid) [38, 39] | 0.007176 | 0.007164 | 0.007109 |
| M062X (mGGA hybrid) [40] | 0.008772 | 0.008706 | 0.008708 |
| M06HF (mGGA hybrid) [40] | 0.008801 | 0.008670 | 0.008765 |
| M06 (mGGA hybrid) [40] | 0.007231 | 0.008603 | 0.007170 |
| Best Estimate [1] | 0.006785 | 0.006796 | 0.006994 |
| Best Estimate [42] | 0.007199889 | 0.00675932 | 0.00652818 |

Table 8: $O_2$ vibrational frequency anharmonicity correction $x_e\omega_e$ (Ha) calculated with different functionals and the DEF2-TZVPP basis set using the Morse function formula $E_n = \omega_e(n+1/2) - (\omega_e^2/4D_e)(n+1/2)^2$ (so $x_e\omega_e = \omega_e^2/4D_e$.) (1 Ha = 219474.6 $cm^{-1}$.)

| Functional | $X\,^1\Sigma_g^-$ | $a\,^1\Delta_g$ | $b\,^1\Sigma_g^+$ |
|---|---|---|---|
| X$\alpha$ = 0.75 [3] | 0.00006750 | 0.00008311 | 0.00010499 |
| Hartree-Fock [4] | 0.00079651 | -0.00099602 | -0.00030272 |
| VWN (LDA) [5, 6] | 0.00004475 | 0.00005087 | 0.00006235 |
| PZ81 (LDA) [5, 7] | 0.00004420 | 0.00004975 | 0.00006045 |
| PW92 (LDA) [5, 8] | 0.00004474 | 0.00005083 | 0.00006228 |
| BLYP (GGA) [9, 10, 11] | 0.00005809 | 0.00006620 | 0.00009445 |
| PW86 (GGA) [12, 13] | 0.00005687 | 0.00006360 | 0.00009392 |
| OLYP (GGA) [10, 14, 11] | 0.00005080 | 0.00006924 | 0.00009449 |
| PW91 (GGA) [15] | 0.00005497 | 0.00006238 | 0.00008867 |
| PW91SSF (GGA) [15] | 0.00005497 | 0.00006238 | 0.00008867 |
| PBE (GGA) [16, 17] | 0.00005507 | 0.00006251 | 0.00008894 |
| PBESSF (GGA) [16, 17] | 0.00005507 | 0.00006251 | 0.00008894 |
| PBSOL (GGA) [18, 19] | 0.00005095 | 0.00005807 | 0.00007772 |
| KT1 (GGA) [20, 21] | 0.00006079 | 0.00006957 | 0.00009451 |
| KT2 (GGA) [20, 21] | 0.00006303 | 0.00007651 | 0.00010853 |
| KT3 (GGA) [20, 21] | 0.00006347 | 0.00007734 | 0.00011155 |
| SO11 (GGA) [22] | 0.00005711 | 0.00006640 | 0.00009489 |
| N12 (GGA) [23] | 0.00006222 | 0.00007623 | 0.00010623 |
| GAM (GGA) [24] | 0.00005792 | 0.00007217 | 0.00009534 |
| CAP (GGA) [25] | 0.00005744 | 0.00006639 | 0.00009526 |
| VS98 (mGGA) [26, 27] | 0.00006214 | 0.00007718 | 0.00010536 |
| PKZB (mGGA) [28, 29] | 0.00006228 | 0.00007262 | 0.00010352 |
| TPSS (mGGA) [30, 31] | 0.00006258 | 0.00007134 | 0.00011102 |
| M06L (mGGA) [32] | 0.00006643 | 0.00008223 | 0.00011151 |
| M11L (mGGA) [33] | 0.00006479 | 0.00008011 | 0.00010480 |
| MN12 (mGGA) [34] | 0.00007196 | 0.00010533 | 0.00010194 |
| B3LYP (hybrid) [35, 36] | 0.00006534 | 0.00007666 | 0.00011294 |
| BH&H (hybrid) [37] | 0.00012299 | 0.00015580 | 0.00027120 |
| PBE0 (hybrid) [38, 39] | 0.00006544 | 0.00007737 | 0.00011834 |
| M062X (mGGA hybrid) [40] | 0.00010063 | 0.00012234 | 0.00015567 |
| M06HF (mGGA hybrid) [40] | 0.00011550 | 0.00013574 | 0.00017538 |
| M06 (mGGA hybrid) [40] | 0.00006609 | 0.00012002 | 0.00009854 |
| Best Estimate [1] | 0.00005946 | 0.0000736 | 0.00009190 |
| Best Estimate [42] | 0.000054589 | 0.0000588 | 0.00006379 |

# 6 Author Contributions

Team members in Cameroon :

- Abraham Ponra, PhD Student, University of Maroua: Carried out the majority of the calculations with the different functionals.
- Prof. Anne Justine Etindele: Thesis Advisor, PhD senior Lecturer, Higher Teachers Training College University of Yaounde I, P.O. Box 47 Yaounde, Cameroon: Worked closely directing AP, carried out some of the calculations, and contributed to the writing of this article.
- Prof. Ousmanou Motapon: Supervisor, Professor, University of Maroua: Follows and is responsible for regularly monitoring the progress of AP's PhD project. He gave a particularly careful reading of a nearly finalized version of the manuscript.

Team members in Grenoble :

- Mark E. Casida: Project design, theory, writing, and some of the calculations.

All authors have read a nearly final version of, and contributed comments and suggestions towards improving, the final manuscript.

# References


[1] Z. Farooq, D. A. Chestakov, B. Yan, G. C. Groenenboom, W. J. van der Zande, and D. H. Parker, Photodissociation of singlet oxygen in the UV region, Phys. Chem. Chem. Phys. **16**, 3305 (2014).

[2] A. Rohatgi, WebPlotDigitizer: Webbased plot digitizer, https://apps.automeris.io/wpd/, Last accessed 3 June 2021.

[3] J. C. Slater, A simplification of the Hartree-Fock method, Phys. Rev. **81**, 3455 (1951).

[4] D. Mejía-Rodriguez and A. M. Köster, Robust and efficient variational fitting of Fock exchange, J. Chem. Phys. **141**, 124114 (2014).

[5] P. A. M. Dirac, Note on exchange phenomena in the Thomas atom, Proc. Camb. Phil. Soc. **26**, 376 (1930).

[6] S. H. Vosko, L. Wilk, and M. Nusair, Accurate spin-dependent electron liquid correlation energies for local spin density calculations: a critical analysis, Can. J. Phys. **58**, 1200 (1980).

[7] J. P. Perdew and A. Zunger, Self-interaction correction to density-functional approximations for many-electron systems, Phys. Rev. B **23**, 5048 (1981).

[8] J. P. Perdew and Y. Wang, Accurate and simple analytic representation of the electron-gas correlation energy, Phys. Rev. B **45**, 13244 (1992).

[9] R. Colle and D. Salvetti, Approximate calculation of the correlation energy for the closed shells, Theor. Chim. Acta **37**, 329 (1975).

[10] R. Colle and D. Salvetti, A general method for approximating the electronic correlation energy in molecules and solids, J. Chem. Phys. **79**, 1404 (1983).

[11] C. Lee, W. Yang, and R. G. Parr, Development of the Colle-Salvetti correlation-energy formula into a functional of the electron density, Phys. Rev. B **37**, 785 (1988).

[12] J. P. Perdew, Density-functional approximation for the correlation energy of the inhomogeneous electron gas, Phys. Rev. B **33**, 8822(R) (1986).

[13] J. P. Perdew, Erratum: Density-functional approximation for the correlation energy of the inhomogeneous electron gas, Phys. Rev. B **34**, 7406 (1986).

[14] A. D. Becke, Density-functional exchange-energy approximation with correct asymptotic behavior, Phys. Rev. A **38**, 3098 (1988).

[15] J. P. Perdew, J. A. Chevary, S. H. Vosko, K. A. Jackson, M. R. Pederson, D. J. Singh, and C. Fiolhais, Atoms, molecules, solids, and surfaces: Applications of the generalized gradient approximation for exchange and correlation, Phys. Rev. B **46**, 6671 (1992).

[16] J. P. Perdew, K. Burke, and M. Ernzerhof, Generalized gradient approximation made simple, Phys. Rev. Lett. **77**, 3865 (1996).

[17] J. P. Perdew, K. Burke, and M. Ernzerhof, Generalized gradient approximation made simple [Phys. Rev. Lett. 77, 3865 (1996)], Phys. Rev. Lett. **78**, 1396(E) (1997).

[18] J. P. Perdew, A. Ruzsinszky, G. I. Csonka, O. A. Vydrov, G. E. Scuseria, L. A. Constantin, X. Zhou, and K. Burke, Restoring the density-gradient expansion for exchange in solids and surfaces, Phys. Rev. Lett. **100**, 136406 (2008).

[19] J. P. Perdew, A. Ruzsinszky, G. I. Csonka, O. A. Vydrov, G. E. Scuseria, L. A. Constantin, X. Zhou, and K. Burke, Erratum: Restoring the density-gradient expansion for exchange in solids and surfaces [*phys. rev. lett.* **100**, 136406 (2008)], Phys. Rev. Lett. **102**, 039902 (2009).

[20] T. W. Keal and D. J. Tozer, The exchange-correlation potential in KohnSham nuclear magnetic resonance shielding calculations, J. Chem. Phys. **119**, 3015 (2003).

[21] T. W. Keal and D. J. Tozer, A semiempirical generalized gradient approximation exchange-correlation functional, J. Chem. Phys. **121**, 5654 (2004).

[22] R. Peverati, Y. Zhao, and D. G. Truhlar, Generalized gradient approximation that recovers the second-order density-gradient expansion with optimized across-the-board performance, J. Phys. Chem. Lett. **2**, 1991 (2011).

[23] R. Peverati and D. G. Truhlar, Exchange-correlation functional with good accuracy for both structural and energetic properties while depending only on the density and its gradient, J. Chem. Theor. Comput. **8**, 2310 (2012).

[24] H. S. Yu, W. Zhang, P. Verma, Z. He, and D. G. Truhlar, Nonseparable exchange-correlation functional for molecules, including homogeneous catalysis involving transition metals, Phys. Chem. Chem. Phys. **17**, 12146 (2015).

[25] J. Carmona-Espíndola, J. L. Gázquez, A. Vela, and S. B. Trickey, Generalized gradient approximation exchange energy functional with correct asymptotic behavior of the corresponding potential, J. Chem. Phys. **142**, 054105 (2015).

[26] T. van Voorhis and G. E. Scuseria, A novel form for the exchange-correlation energy functional, J. Chem. Phys. **109**, 400 (1998).

[27] T. van Voorhis and G. E. Scuseria, Erratum: "A novel form for the exchange-correlation energy functional" [*j. chem. phys.* **109**, 400 (1998)], J. Chem. Phys. **129**, 219901 (2008).

[28] J. P. Perdew, S. Kurth, A. Zupan, and P. Blaha, Accurate density functional with correct formal properties: A step beyond the generalized gradient approximation, Phys. Rev. Lett. **82**, 2544 (1999).

[29] J. P. Perdew, S. Kurth, A. Zupan, and P. Blaha, Erratum: Accurate density functional with correct formal properties: A step beyond the generalized gradient approximation [*phys. rev. lett.* **82**, 2544 (1999)], Phys. Rev. Lett. **82**, 5197 (1999).

[30] J. Tao, J. P. Perdew, V. N. Staroverov, and G. E. Scuseria, Climbing the density functional ladder: Nonempirical meta-generalized gradient approximation designed for molecules and solids, Phys. Rev. Lett. **91**, 146401 (2003).

[31] J. Tao, J. P. Perdew, V. N. Staroverov, and G. E. Scuseria, Meta-generalized gradient approximation: Explanation of a realistic nonempirical density functional, J. Chem. Phys. **120**, 6898 (2004).

[32] Y. Zhao and D. G. Truhlar, A new local density functional for main-group thermochemistry, transition metal bonding, thermochemical kinetics, and noncovalent interactions, J. Chem. Phys. **125**, 194101 (2006).

[33] R. Peverati and D. G. Truhlar, M11-L: A local density functional that provides improved accuracy for electronic structure calculations in chemistry and physics, J. Phys. Chem. Lett. **3**, 117 (2012).

[34] R. Peverati and D. G. Truhlar, An improved and broadly accurate local approximation to the exchange-correlation density functional: The MN12-L functional for electronic structure calculations in chemistry and physics, Phys. Chem. Chem. Phys. **14**, 13171 (2012).

[35] A. D. Becke, Density-functional thermochemistry. III. The role of exact exchange, J. Chem. Phys. **98**, 5648 (1993).

[36] P. J. Stephens, F. J. Devlin, C. Chabalowski, and M. Frisch, Ab initio calculation of vibrational absorption and circular dichroism spectra using density functional force fields, J. Chem. Phys. **98**, 11623 (1994).

[37] A. D. Becke, A new mixing of Hartree-Fock and local densityfunctional theories, J. Chem. Phys. **98**, 1372 (1993).

[38] J. P. Perdew, M. Ernzerhof, and K. Burke, Rationale for mixing exact exchange with density functional approximations, J. Chem. Phys. **105**, 9982 (1996).

[39] C. Adamo and V. Barone, Toward reliable density functional methods without adjustable parameters: The PBE0 model, J. Chem. Phys. **110**, 6158 (1999).

[40] Y. Zhao and D. G. Truhlar, The M06 suite of density functionals for main group thermochemistry, thermochemical kinetics, noncovalent interactions, excited states, and transition elements: two new functionals and systematic testing of four M06-class functionals and 12 other functionals, Theor. Chem. Acc. **120**, 215 (2007).

[41] D. P. O'Neill and P. M. W. Gill, Benchmark correlation energies for small molecules, Mol. Phys. **103**, 763 (2005).

[42] National institute of standards and technologies atomic spectra database, https://physics.nist.gov/PhysRefData/ASD/levels_form.html, Last accessed 22 June 2021.
